# Supplementary material for: Calibrating Panoramic Depth Estimation for Practical Localization and Mapping
Source: arXiv:2308.14005 source file (2024-02-02)
Supplement: Supplementary file 1 [file supp_full_aggregated.tex]

\begin{table*}[t]
\centering
\resizebox{0.9\linewidth}{!}{
\begin{tabularx}{2.5\columnwidth}{l|YYYYYYYY}
\toprule
\multirow{2}{*}{Method} & \multirow{2}{*}{MAE} & \multirow{2}{*}{Abs. Rel.} & \multirow{2}{*}{Sq. Rel.} & \multirow{2}{*}{RMSE} & \multirow{2}{*}{RMSE (Log)} & Inlier Ratio & Inlier Ratio & Inlier Ratio \\
& & & & & & ($\lambda=1.25$) & ($\lambda=1.25^2$)& ($\lambda=1.25^3$)\\
\midrule
No Adaptation & 0.4460 & 0.2163 & 0.1705 & 0.6222 & 0.1053 & 0.6960 & 0.9412 & 0.9801 \\
Schneider et al.~\cite{batchnorm_update} & 0.5226 & 0.2296 & 0.2340 & 0.7984 & 0.1254 & 0.6334 & 0.9006 & 0.9599 \\
Tent~\cite{tent} & 0.4418 & 0.2143 & 0.1684 & 0.6173 & 0.1046 & 0.7028 & 0.9416 & 0.9803 \\
Flip Consistency & 0.4349 & 0.2104 & 0.1625 & 0.6132 & 0.1028 & 0.7035 & 0.9417 & 0.9804 \\
Mask Consistency & 0.4153 & 0.2005 & 0.1513 & 0.5910 & 0.0996 & 0.7361 & 0.9437 & 0.9811 \\
Photometric Consistency & 0.4467 & 0.2187 & 0.1703 & 0.6222 & 0.1055 & 0.6861 & 0.9425 & 0.9807 \\
Pseudo Labelling & 0.4235 & 0.2068 & 0.1558 & 0.5923 & 0.1012 & 0.7157 & 0.9445 & 0.9819 \\
Vanilla T\textsuperscript{2}Net~\cite{t2net} & 0.4267 & 0.2018 & 0.1567 & 0.6208 & 0.1021 & 0.7320 & 0.9390 & 0.9792 \\
CrDoCo~\cite{chen2019crdoco} & 0.4229 & 0.2041 & 0.1531 & 0.5987 & 0.1012 & 0.7266 & 0.9424 & 0.9810 \\
Feature Consistency & 0.4237 & 0.1996 & 0.1533 & 0.6158 & 0.1013 & 0.7359 & 0.9400 & 0.9795 \\
Ground-Truth Training & 0.3490 & 0.1725 & 0.1196 & 0.5180 & 0.0895 & 0.7965 & 0.9565 & 0.9854 \\
Ours & 0.3653 & 0.1798 & 0.1297 & 0.5253 & 0.0921 & 0.7910 & 0.9512 & 0.9834 \\
\bottomrule
\end{tabularx}
}
\caption{Full aggregated results for offline adaptation using 5\% of the panorama images for training}
\end{table*}

    \smallskip

\begin{table*}[t]
\centering
\resizebox{0.9\linewidth}{!}{
\begin{tabularx}{2.5\columnwidth}{l|YYYYYYYY}
\toprule
\multirow{2}{*}{Method} & \multirow{2}{*}{MAE} & \multirow{2}{*}{Abs. Rel.} & \multirow{2}{*}{Sq. Rel.} & \multirow{2}{*}{RMSE} & \multirow{2}{*}{RMSE (Log)} & Inlier Ratio & Inlier Ratio & Inlier Ratio \\
& & & & & & ($\lambda=1.25$) & ($\lambda=1.25^2$)& ($\lambda=1.25^3$)\\
\midrule
No Adaptation & 0.4443 & 0.2157 & 0.1699 & 0.6232 & 0.1054 & 0.6973 & 0.9422 & 0.9802 \\
Schneider et al.~\cite{batchnorm_update} & 0.5186 & 0.2280 & 0.2302 & 0.7932 & 0.1241 & 0.6336 & 0.9037 & 0.9614 \\
Tent~\cite{tent} & 0.4399 & 0.2136 & 0.1676 & 0.6183 & 0.1046 & 0.7052 & 0.9428 & 0.9803 \\
Flip Consistency & 0.4223 & 0.2057 & 0.1564 & 0.5987 & 0.1013 & 0.7174 & 0.9435 & 0.9809 \\
Mask Consistency & 0.4190 & 0.2018 & 0.1539 & 0.5994 & 0.1009 & 0.7345 & 0.9426 & 0.9804 \\
Photometric Consistency & 0.4394 & 0.2149 & 0.1667 & 0.6123 & 0.1043 & 0.6978 & 0.9440 & 0.9810 \\
Pseudo Labelling & 0.4296 & 0.2076 & 0.1588 & 0.6107 & 0.1027 & 0.7149 & 0.9431 & 0.9807 \\
Vanilla T\textsuperscript{2}Net~\cite{t2net} & 0.4294 & 0.2027 & 0.1588 & 0.6290 & 0.1030 & 0.7307 & 0.9377 & 0.9785 \\
CrDoCo~\cite{chen2019crdoco} & 0.4239 & 0.2045 & 0.1548 & 0.6045 & 0.1018 & 0.7268 & 0.9420 & 0.9806 \\
Feature Consistency & 0.4277 & 0.2005 & 0.1578 & 0.6291 & 0.1028 & 0.7345 & 0.9373 & 0.9781 \\
Ground-Truth Training & 0.3398 & 0.1703 & 0.1167 & 0.5019 & 0.0882 & 0.8039 & 0.9580 & 0.9857 \\
Ours & 0.3620 & 0.1784 & 0.1291 & 0.5231 & 0.0920 & 0.7951 & 0.9511 & 0.9830 \\
\bottomrule
\end{tabularx}
}
\caption{Full aggregated results for offline adaptation using 10\% of the panorama images for training}
\end{table*}

    \smallskip

\begin{table*}[t]
\centering
\resizebox{0.9\linewidth}{!}{
\begin{tabularx}{2.5\columnwidth}{l|YYYYYYYY}
\toprule
\multirow{2}{*}{Method} & \multirow{2}{*}{MAE} & \multirow{2}{*}{Abs. Rel.} & \multirow{2}{*}{Sq. Rel.} & \multirow{2}{*}{RMSE} & \multirow{2}{*}{RMSE (Log)} & Inlier Ratio & Inlier Ratio & Inlier Ratio \\
& & & & & & ($\lambda=1.25$) & ($\lambda=1.25^2$)& ($\lambda=1.25^3$)\\
\midrule
No Adaptation & 0.4412 & 0.2143 & 0.1675 & 0.6211 & 0.1053 & 0.7012 & 0.9424 & 0.9804 \\
Schneider et al.~\cite{batchnorm_update} & 0.4178 & 0.1859 & 0.1593 & 0.7212 & 0.1077 & 0.7427 & 0.9403 & 0.9789 \\
Tent~\cite{tent} & 0.4274 & 0.2044 & 0.1582 & 0.6457 & 0.1052 & 0.7329 & 0.9437 & 0.9805 \\
Flip Consistency & 0.4414 & 0.2037 & 0.1594 & 0.7375 & 0.1092 & 0.7115 & 0.9314 & 0.9745 \\
Mask Consistency & 0.4601 & 0.2170 & 0.1679 & 0.7523 & 0.1130 & 0.6652 & 0.9258 & 0.9723 \\
Photometric Consistency & 0.4595 & 0.2354 & 0.1735 & 0.6633 & 0.1120 & 0.6254 & 0.9355 & 0.9807 \\
Pseudo Labelling & 0.4344 & 0.2143 & 0.1537 & 0.6812 & 0.1085 & 0.6824 & 0.9358 & 0.9774 \\
Vanilla T\textsuperscript{2}Net~\cite{t2net} & 0.4022 & 0.1984 & 0.1421 & 0.6303 & 0.1024 & 0.7471 & 0.9408 & 0.9791 \\
CrDoCo~\cite{chen2019crdoco} & 0.4646 & 0.2191 & 0.1727 & 0.7665 & 0.1139 & 0.6663 & 0.9245 & 0.9708 \\
Feature Consistency & 0.6412 & 0.2511 & 0.3080 & 1.1059 & 0.1683 & 0.5686 & 0.8090 & 0.9028 \\
Ground-Truth Training & 0.2388 & 0.1110 & 0.0736 & 0.4351 & 0.0713 & 0.8846 & 0.9719 & 0.9903 \\
Ours & 0.3234 & 0.1494 & 0.1045 & 0.5246 & 0.0865 & 0.8300 & 0.9607 & 0.9872
 \\
\bottomrule
\end{tabularx}
}
\caption{Full aggregated results for online adaptation in dataset shift}
\end{table*}

    \smallskip

\begin{table*}[t]
\centering
\resizebox{0.9\linewidth}{!}{
\begin{tabularx}{2.5\columnwidth}{l|YYYYYYYY}
\toprule
\multirow{2}{*}{Method} & \multirow{2}{*}{MAE} & \multirow{2}{*}{Abs. Rel.} & \multirow{2}{*}{Sq. Rel.} & \multirow{2}{*}{RMSE} & \multirow{2}{*}{RMSE (Log)} & Inlier Ratio & Inlier Ratio & Inlier Ratio \\
& & & & & & ($\lambda=1.25$) & ($\lambda=1.25^2$)& ($\lambda=1.25^3$)\\
\midrule
No Adaptation & 0.3862 & 0.2185 & 0.1480 & 0.5135 & 0.1039 & 0.6848 & 0.9516 & 0.9836 \\
Schneider et al.~\cite{batchnorm_update} & 0.4075 & 0.2255 & 0.1597 & 0.5643 & 0.1035 & 0.6778 & 0.9505 & 0.9852 \\
Tent~\cite{tent} & 0.3653 & 0.2072 & 0.1349 & 0.5011 & 0.1022 & 0.7276 & 0.9542 & 0.9843 \\
Flip Consistency & 0.3040 & 0.1864 & 0.0978 & 0.4087 & 0.0942 & 0.7753 & 0.9591 & 0.9867 \\
Mask Consistency & 0.3246 & 0.2053 & 0.1057 & 0.4231 & 0.1001 & 0.7121 & 0.9537 & 0.9861 \\
Photometric Consistency & 0.3634 & 0.2132 & 0.1325 & 0.4840 & 0.1054 & 0.6909 & 0.9510 & 0.9828 \\
Pseudo Labelling & 0.3564 & 0.2219 & 0.1235 & 0.4543 & 0.1041 & 0.6781 & 0.9509 & 0.9855 \\
Vanilla T\textsuperscript{2}Net~\cite{t2net} & 0.3433 & 0.2215 & 0.1213 & 0.4334 & 0.1045 & 0.6962 & 0.9484 & 0.9844 \\
CrDoCo~\cite{chen2019crdoco} & 0.3347 & 0.2081 & 0.1090 & 0.4445 & 0.1022 & 0.7055 & 0.9504 & 0.9853 \\
Feature Consistency & 0.4775 & 0.2459 & 0.2082 & 0.7111 & 0.1480 & 0.5827 & 0.8413 & 0.9292 \\
Ground-Truth Training & 0.1912 & 0.1125 & 0.0545 & 0.2984 & 0.0695 & 0.8855 & 0.9724 & 0.9911 \\
Ours & 0.2362 & 0.1333 & 0.0690 & 0.3605 & 0.0779 & 0.8584 & 0.9692 & 0.9894 \\
\bottomrule
\end{tabularx}
}
\caption{Full aggregated results for online adaptation in low lighting}
\end{table*}

\begin{table*}[t]
\centering
\resizebox{0.9\linewidth}{!}{
\begin{tabularx}{2.5\columnwidth}{l|YYYYYYYY}
\toprule
\multirow{2}{*}{Method} & \multirow{2}{*}{MAE} & \multirow{2}{*}{Abs. Rel.} & \multirow{2}{*}{Sq. Rel.} & \multirow{2}{*}{RMSE} & \multirow{2}{*}{RMSE (Log)} & Inlier Ratio & Inlier Ratio & Inlier Ratio \\
& & & & & & ($\lambda=1.25$) & ($\lambda=1.25^2$)& ($\lambda=1.25^3$)\\
\midrule
No Adaptation & 0.4141 & 0.2325 & 0.1615 & 0.5441 & 0.1110 & 0.6454 & 0.9404 & 0.9781 \\
Schneider et al.~\cite{batchnorm_update} & 0.4089 & 0.2256 & 0.1588 & 0.5636 & 0.1034 & 0.6742 & 0.9511 & 0.9857 \\
Tent~\cite{tent} & 0.3926 & 0.2207 & 0.1481 & 0.5342 & 0.1100 & 0.6901 & 0.9433 & 0.9788 \\
Flip Consistency & 0.3216 & 0.1904 & 0.1041 & 0.4472 & 0.1003 & 0.7608 & 0.9481 & 0.9807 \\
Mask Consistency & 0.3378 & 0.2118 & 0.1109 & 0.4395 & 0.1024 & 0.6995 & 0.9504 & 0.9853 \\
Photometric Consistency & 0.4190 & 0.2492 & 0.1597 & 0.5321 & 0.1153 & 0.5810 & 0.9396 & 0.9804 \\
Pseudo Labelling & 0.3673 & 0.2295 & 0.1281 & 0.4615 & 0.1069 & 0.6636 & 0.9456 & 0.9840 \\
Vanilla T\textsuperscript{2}Net~\cite{t2net} & 0.3592 & 0.2263 & 0.1262 & 0.4514 & 0.1057 & 0.6888 & 0.9478 & 0.9844 \\
CrDoCo~\cite{chen2019crdoco} & 0.3379 & 0.2125 & 0.1105 & 0.4394 & 0.1026 & 0.7026 & 0.9504 & 0.9856 \\
Feature Consistency & 0.4901 & 0.2495 & 0.2149 & 0.7294 & 0.1538 & 0.5703 & 0.8295 & 0.9242 \\
Ground-Truth Training & 0.1916 & 0.1126 & 0.0541 & 0.3003 & 0.0698 & 0.8855 & 0.9720 & 0.9908 \\
Ours & 0.2527 & 0.1393 & 0.0749 & 0.3892 & 0.0834 & 0.8437 & 0.9627 & 0.9860
 \\
\bottomrule
\end{tabularx}
}
\caption{Full aggregated results for online adaptation in white balance change}
\end{table*}

\begin{table*}[t]
\centering
\resizebox{0.9\linewidth}{!}{
\begin{tabularx}{2.5\columnwidth}{l|YYYYYYYY}
\toprule
\multirow{2}{*}{Method} & \multirow{2}{*}{MAE} & \multirow{2}{*}{Abs. Rel.} & \multirow{2}{*}{Sq. Rel.} & \multirow{2}{*}{RMSE} & \multirow{2}{*}{RMSE (Log)} & Inlier Ratio & Inlier Ratio & Inlier Ratio \\
& & & & & & ($\lambda=1.25$) & ($\lambda=1.25^2$)& ($\lambda=1.25^3$)\\
\midrule
No Adaptation & 0.4048 & 0.2312 & 0.1565 & 0.5245 & 0.1048 & 0.6817 & 0.9489 & 0.9841 \\
Schneider et al.~\cite{batchnorm_update} & 0.4062 & 0.2242 & 0.1552 & 0.5587 & 0.1027 & 0.6768 & 0.9522 & 0.9861 \\
Tent~\cite{tent} & 0.3792 & 0.2173 & 0.1413 & 0.5046 & 0.1022 & 0.7266 & 0.9524 & 0.9851 \\
Flip Consistency & 0.3292 & 0.2072 & 0.1089 & 0.4191 & 0.0983 & 0.7360 & 0.9560 & 0.9868 \\
Mask Consistency & 0.3341 & 0.2121 & 0.1079 & 0.4271 & 0.1008 & 0.6975 & 0.9549 & 0.9870 \\
Photometric Consistency & 0.4192 & 0.2597 & 0.1717 & 0.5157 & 0.1144 & 0.5920 & 0.9373 & 0.9816 \\
Pseudo Labelling & 0.3506 & 0.2202 & 0.1187 & 0.4383 & 0.1018 & 0.7043 & 0.9530 & 0.9863 \\
Vanilla T\textsuperscript{2}Net~\cite{t2net} & 0.3338 & 0.2138 & 0.1157 & 0.4229 & 0.1007 & 0.7275 & 0.9518 & 0.9852 \\
CrDoCo~\cite{chen2019crdoco} & 0.3284 & 0.2096 & 0.1079 & 0.4246 & 0.1000 & 0.7255 & 0.9527 & 0.9862 \\
Feature Consistency & 0.3985 & 0.2103 & 0.1518 & 0.5914 & 0.1230 & 0.6646 & 0.8945 & 0.9620 \\
Ground-Truth Training & 0.1830 & 0.1076 & 0.0520 & 0.2904 & 0.0672 & 0.8962 & 0.9742 & 0.9915 \\
Ours & 0.2332 & 0.1308 & 0.0672 & 0.3599 & 0.0766 & 0.8666 & 0.9705 & 0.9898
 \\
\bottomrule
\end{tabularx}
}
\caption{Full aggregated results for online adaptation in image gamma change}
\end{table*}

\begin{table*}[t]
\centering
\resizebox{0.9\linewidth}{!}{
\begin{tabularx}{2.5\columnwidth}{l|YYYYYYYY}
\toprule
\multirow{2}{*}{Method} & \multirow{2}{*}{MAE} & \multirow{2}{*}{Abs. Rel.} & \multirow{2}{*}{Sq. Rel.} & \multirow{2}{*}{RMSE} & \multirow{2}{*}{RMSE (Log)} & Inlier Ratio & Inlier Ratio & Inlier Ratio \\
& & & & & & ($\lambda=1.25$) & ($\lambda=1.25^2$)& ($\lambda=1.25^3$)\\
\midrule
No Adaptation & 0.4950 & 0.1892 & 0.1829 & 0.7659 & 0.1054 & 0.7289 & 0.9341 & 0.9751 \\
Schneider et al.~\cite{batchnorm_update} & 0.6117 & 0.2002 & 0.2547 & 1.0768 & 0.1429 & 0.6604 & 0.8783 & 0.9495 \\
Tent~\cite{tent} & 0.5021 & 0.1887 & 0.1845 & 0.8251 & 0.1093 & 0.7296 & 0.9321 & 0.9745 \\
Flip Consistency & 0.5491 & 0.1913 & 0.2019 & 0.9298 & 0.1123 & 0.7160 & 0.9180 & 0.9677 \\
Mask Consistency & 0.5451 & 0.1922 & 0.1971 & 0.9296 & 0.1100 & 0.7177 & 0.9200 & 0.9710 \\
Photometric Consistency & 0.5097 & 0.1936 & 0.1844 & 0.8308 & 0.1097 & 0.6993 & 0.9344 & 0.9761 \\
Pseudo Labelling & 0.5160 & 0.1876 & 0.1810 & 0.8770 & 0.1071 & 0.7269 & 0.9279 & 0.9751 \\
Vanilla T\textsuperscript{2}Net~\cite{t2net} & 0.5268 & 0.1843 & 0.1874 & 0.9118 & 0.1076 & 0.7399 & 0.9241 & 0.9720 \\
CrDoCo~\cite{chen2019crdoco} & 0.5554 & 0.1905 & 0.2032 & 0.9755 & 0.1111 & 0.7230 & 0.9164 & 0.9680 \\
Feature Consistency & 0.7215 & 0.2214 & 0.3261 & 1.2991 & 0.1578 & 0.6197 & 0.8368 & 0.9197 \\
Ground-Truth Training & 0.3437 & 0.1320 & 0.1135 & 0.6072 & 0.0804 & 0.8599 & 0.9665 & 0.9879 \\
Ours & 0.4239 & 0.1591 & 0.1430 & 0.6977 & 0.0931 & 0.8032 & 0.9525 & 0.9844
 \\
\bottomrule
\end{tabularx}
}
\caption{Full aggregated results for online adaptation in large scenes}
\end{table*}

\begin{table*}[t]
\centering
\resizebox{0.9\linewidth}{!}{
\begin{tabularx}{2.5\columnwidth}{l|YYYYYYYY}
\toprule
\multirow{2}{*}{Method} & \multirow{2}{*}{MAE} & \multirow{2}{*}{Abs. Rel.} & \multirow{2}{*}{Sq. Rel.} & \multirow{2}{*}{RMSE} & \multirow{2}{*}{RMSE (Log)} & Inlier Ratio & Inlier Ratio & Inlier Ratio \\
& & & & & & ($\lambda=1.25$) & ($\lambda=1.25^2$)& ($\lambda=1.25^3$)\\
\midrule
No Adaptation & 0.3116 & 0.1770 & 0.0975 & 0.4292 & 0.0887 & 0.7878 & 0.9573 & 0.9872 \\
Schneider et al.~\cite{batchnorm_update} & 0.4010 & 0.2347 & 0.1911 & 0.5508 & 0.1021 & 0.6841 & 0.9103 & 0.9768 \\
Tent~\cite{tent} & 0.3071 & 0.1743 & 0.0953 & 0.4282 & 0.0889 & 0.7938 & 0.9577 & 0.9873 \\
Flip Consistency & 0.3049 & 0.1772 & 0.0899 & 0.4105 & 0.0890 & 0.7847 & 0.9618 & 0.9879 \\
Mask Consistency & 0.2724 & 0.1646 & 0.0781 & 0.3666 & 0.0835 & 0.8059 & 0.9657 & 0.9894 \\
Photometric Consistency & 0.2900 & 0.1700 & 0.0904 & 0.3995 & 0.0858 & 0.7962 & 0.9584 & 0.9877 \\
Pseudo Labelling & 0.3000 & 0.1764 & 0.0906 & 0.4033 & 0.0864 & 0.7907 & 0.9623 & 0.9889 \\
Vanilla T\textsuperscript{2}Net~\cite{t2net} & 0.2743 & 0.1674 & 0.0806 & 0.3674 & 0.0843 & 0.7996 & 0.9643 & 0.9890 \\
CrDoCo~\cite{chen2019crdoco} & 0.2629 & 0.1598 & 0.0741 & 0.3576 & 0.0826 & 0.8121 & 0.9643 & 0.9885 \\
Feature Consistency & 0.2881 & 0.1606 & 0.0831 & 0.4089 & 0.0902 & 0.7829 & 0.9541 & 0.9836 \\
Ground-Truth Training & 0.2168 & 0.1299 & 0.0592 & 0.3122 & 0.0725 & 0.8575 & 0.9688 & 0.9897 \\
Ours & 0.2440 & 0.1420 & 0.0674 & 0.3498 & 0.0780 & 0.8351 & 0.9657 & 0.9888
 \\
\bottomrule
\end{tabularx}
}
\caption{Full aggregated results for online adaptation in small scenes}
\end{table*}

\begin{table*}[t]
\centering
\resizebox{0.9\linewidth}{!}{
\begin{tabularx}{2.5\columnwidth}{l|YYYYYYYY}
\toprule
\multirow{2}{*}{Method} & \multirow{2}{*}{MAE} & \multirow{2}{*}{Abs. Rel.} & \multirow{2}{*}{Sq. Rel.} & \multirow{2}{*}{RMSE} & \multirow{2}{*}{RMSE (Log)} & Inlier Ratio & Inlier Ratio & Inlier Ratio \\
& & & & & & ($\lambda=1.25$) & ($\lambda=1.25^2$)& ($\lambda=1.25^3$)\\
\midrule
No Adaptation & 0.5254 & 0.3275 & 0.3367 & 0.7433 & 0.1611 & 0.5327 & 0.8073 & 0.9163 \\
Schneider et al.~\cite{batchnorm_update} & 0.5562 & 0.3355 & 0.3704 & 0.7965 & 0.1669 & 0.4781 & 0.7927 & 0.9177 \\
Tent~\cite{tent} & 0.5076 & 0.3133 & 0.3088 & 0.7228 & 0.1585 & 0.5461 & 0.8163 & 0.9216 \\
Flip Consistency & 0.4524 & 0.2730 & 0.2106 & 0.6588 & 0.1417 & 0.5770 & 0.8534 & 0.9439 \\
Mask Consistency & 0.4701 & 0.2777 & 0.2259 & 0.6998 & 0.1472 & 0.5726 & 0.8375 & 0.9348 \\
Photometric Consistency & 0.5348 & 0.3445 & 0.3537 & 0.7358 & 0.1593 & 0.5238 & 0.8095 & 0.9194 \\
Pseudo Labelling & 0.4771 & 0.2821 & 0.2315 & 0.7014 & 0.1488 & 0.5601 & 0.8346 & 0.9349 \\
Vanilla T\textsuperscript{2}Net~\cite{t2net} & 0.4665 & 0.3125 & 0.2742 & 0.6432 & 0.1483 & 0.5751 & 0.8407 & 0.9332 \\
CrDoCo~\cite{chen2019crdoco} & 0.4466 & 0.2570 & 0.2018 & 0.6819 & 0.1414 & 0.6054 & 0.8504 & 0.9415 \\
Feature Consistency & 0.6060 & 0.3031 & 0.3101 & 0.9231 & 0.2019 & 0.4586 & 0.7172 & 0.8539 \\
Ground-Truth Training & 0.3190 & 0.1985 & 0.1354 & 0.4767 & 0.1094 & 0.7300 & 0.9134 & 0.9682 \\
Ours & 0.4402 & 0.2362 & 0.1878 & 0.6684 & 0.1452 & 0.5806 & 0.8419 & 0.9428
 \\
\bottomrule
\end{tabularx}
}
\caption{Full aggregated results for online adaptation in camera rotations}
\end{table*}

\begin{table*}[t]
\centering
\resizebox{0.9\linewidth}{!}{
\begin{tabularx}{2.5\columnwidth}{l|YYYYYYYY}
\toprule
\multirow{2}{*}{Method} & \multirow{2}{*}{MAE} & \multirow{2}{*}{Abs. Rel.} & \multirow{2}{*}{Sq. Rel.} & \multirow{2}{*}{RMSE} & \multirow{2}{*}{RMSE (Log)} & Inlier Ratio & Inlier Ratio & Inlier Ratio \\
& & & & & & ($\lambda=1.25$) & ($\lambda=1.25^2$)& ($\lambda=1.25^3$)\\
\midrule
No Adaptation & 0.5329 & 0.2800 & 0.3145 & 0.7810 & 0.1890 & 0.5648 & 0.7812 & 0.8697 \\
Schneider et al.~\cite{batchnorm_update} & 0.4277 & 0.2406 & 0.1831 & 0.5946 & 0.1106 & 0.6428 & 0.9373 & 0.9801 \\
Tent~\cite{tent} & 0.5126 & 0.2670 & 0.2860 & 0.8028 & 0.1938 & 0.5829 & 0.7914 & 0.8772 \\
Flip Consistency & 0.4357 & 0.2346 & 0.1864 & 0.6433 & 0.1450 & 0.6331 & 0.8665 & 0.9319 \\
Mask Consistency & 0.5178 & 0.2528 & 0.2424 & 0.7889 & 0.1750 & 0.5784 & 0.7921 & 0.8851 \\
Photometric Consistency & 0.4533 & 0.2537 & 0.2450 & 0.6941 & 0.1634 & 0.6299 & 0.8456 & 0.9163 \\
Pseudo Labelling & 0.3995 & 0.2134 & 0.1594 & 0.6116 & 0.1331 & 0.6853 & 0.8834 & 0.9448 \\
Vanilla T\textsuperscript{2}Net~\cite{t2net} & 0.3731 & 0.2216 & 0.1649 & 0.5460 & 0.1264 & 0.7014 & 0.9014 & 0.9554 \\
CrDoCo~\cite{chen2019crdoco} & 0.4582 & 0.2349 & 0.1978 & 0.6924 & 0.1495 & 0.6270 & 0.8460 & 0.9207 \\
Feature Consistency & 0.4329 & 0.2269 & 0.1780 & 0.6653 & 0.1418 & 0.6363 & 0.8647 & 0.9400 \\
Ground-Truth Training & 0.2370 & 0.1391 & 0.0800 & 0.3712 & 0.0868 & 0.8339 & 0.9484 & 0.9799 \\
Ours & 0.3143 & 0.1614 & 0.1074 & 0.5047 & 0.1067 & 0.7701 & 0.9262 & 0.9681
 \\
\bottomrule
\end{tabularx}
}
\caption{Full aggregated results for online adaptation in Gaussian noise}
\end{table*}

\begin{table*}[t]
\centering
\resizebox{0.9\linewidth}{!}{
\begin{tabularx}{2.5\columnwidth}{l|YYYYYYYY}
\toprule
\multirow{2}{*}{Method} & \multirow{2}{*}{MAE} & \multirow{2}{*}{Abs. Rel.} & \multirow{2}{*}{Sq. Rel.} & \multirow{2}{*}{RMSE} & \multirow{2}{*}{RMSE (Log)} & Inlier Ratio & Inlier Ratio & Inlier Ratio \\
& & & & & & ($\lambda=1.25$) & ($\lambda=1.25^2$)& ($\lambda=1.25^3$)\\
\midrule
No Adaptation & 0.7756 & 0.4490 & 0.5792 & 1.0052 & 0.1773 & 0.3425 & 0.7521 & 0.9078 \\
Schneider et al.~\cite{batchnorm_update} & 0.4261 & 0.2369 & 0.1779 & 0.5956 & 0.1098 & 0.6539 & 0.9381 & 0.9815 \\
Tent~\cite{tent} & 0.7220 & 0.4178 & 0.5058 & 0.9506 & 0.1706 & 0.3835 & 0.7831 & 0.9205 \\
Flip Consistency & 0.4734 & 0.2967 & 0.2072 & 0.5884 & 0.1308 & 0.4963 & 0.8950 & 0.9699 \\
Mask Consistency & 0.4774 & 0.3051 & 0.2158 & 0.5936 & 0.1344 & 0.4798 & 0.8873 & 0.9661 \\
Photometric Consistency & 0.8657 & 0.5226 & 0.7008 & 1.0652 & 0.1971 & 0.2345 & 0.6882 & 0.8811 \\
Pseudo Labelling & 0.4986 & 0.3126 & 0.2261 & 0.6096 & 0.1349 & 0.4602 & 0.8883 & 0.9669 \\
Vanilla T\textsuperscript{2}Net~\cite{t2net} & 0.6058 & 0.3934 & 0.3772 & 0.7499 & 0.1620 & 0.4217 & 0.8026 & 0.9305 \\
CrDoCo~\cite{chen2019crdoco} & 0.4115 & 0.2596 & 0.1652 & 0.5325 & 0.1204 & 0.5917 & 0.9140 & 0.9739 \\
Feature Consistency & 0.5007 & 0.2508 & 0.2244 & 0.7620 & 0.1569 & 0.5712 & 0.8241 & 0.9196 \\
Ground-Truth Training & 0.2512 & 0.1471 & 0.0855 & 0.3762 & 0.0830 & 0.8272 & 0.9555 & 0.9855 \\
Ours & 0.3514 & 0.2034 & 0.1313 & 0.4896 & 0.1029 & 0.7025 & 0.9395 & 0.9815
 \\
\bottomrule
\end{tabularx}
}
\caption{Full aggregated results for online adaptation in salt and pepper noise}
\end{table*}

\begin{table*}[t]
\centering
\resizebox{0.9\linewidth}{!}{
\begin{tabularx}{2.5\columnwidth}{l|YYYYYYYY}
\toprule
\multirow{2}{*}{Method} & \multirow{2}{*}{MAE} & \multirow{2}{*}{Abs. Rel.} & \multirow{2}{*}{Sq. Rel.} & \multirow{2}{*}{RMSE} & \multirow{2}{*}{RMSE (Log)} & Inlier Ratio & Inlier Ratio & Inlier Ratio \\
& & & & & & ($\lambda=1.25$) & ($\lambda=1.25^2$)& ($\lambda=1.25^3$)\\
\midrule
No Adaptation & 0.5287 & 0.2896 & 0.3265 & 0.7612 & 0.1785 & 0.5574 & 0.7953 & 0.8889 \\
Schneider et al.~\cite{batchnorm_update} & 0.4343 & 0.2437 & 0.1843 & 0.6044 & 0.1119 & 0.6368 & 0.9342 & 0.9795 \\
Tent~\cite{tent} & 0.5061 & 0.2740 & 0.2866 & 0.7680 & 0.1799 & 0.5765 & 0.8074 & 0.8975 \\
Flip Consistency & 0.4900 & 0.2629 & 0.2202 & 0.6904 & 0.1578 & 0.5531 & 0.8334 & 0.9189 \\
Mask Consistency & 0.4329 & 0.2357 & 0.1770 & 0.6344 & 0.1362 & 0.6195 & 0.8784 & 0.9490 \\
Photometric Consistency & 0.5152 & 0.3087 & 0.3929 & 0.7742 & 0.1784 & 0.5842 & 0.8155 & 0.8960 \\
Pseudo Labelling & 0.4090 & 0.2336 & 0.1734 & 0.6000 & 0.1306 & 0.6469 & 0.8951 & 0.9570 \\
Vanilla T\textsuperscript{2}Net~\cite{t2net} & 0.3907 & 0.2388 & 0.1782 & 0.5495 & 0.1257 & 0.6660 & 0.9057 & 0.9621 \\
CrDoCo~\cite{chen2019crdoco} & 0.4298 & 0.2324 & 0.1736 & 0.6377 & 0.1346 & 0.6311 & 0.8803 & 0.9496 \\
Feature Consistency & 0.4346 & 0.2324 & 0.1786 & 0.6545 & 0.1395 & 0.6190 & 0.8715 & 0.9466 \\
Ground-Truth Training & 0.2428 & 0.1436 & 0.0822 & 0.3743 & 0.0862 & 0.8303 & 0.9539 & 0.9831 \\
Ours & 0.2990 & 0.1653 & 0.0996 & 0.4604 & 0.0974 & 0.7844 & 0.9456 & 0.9799
 \\
\bottomrule
\end{tabularx}
}
\caption{Full aggregated results for online adaptation in speckle noise}
\end{table*}
