# Supplementary material for: Calibrating Panoramic Depth Estimation for Practical Localization and Mapping
Source: arXiv:2308.14005 source file (2024-02-02)
Supplement: Supplementary file 2 [file supp_full_omniscenes.tex]

\begin{table*}[t]
\centering
\resizebox{0.9\linewidth}{!}{
\begin{tabularx}{2.5\columnwidth}{l|YYYYYYYY}
\toprule
\multirow{2}{*}{Method} & \multirow{2}{*}{MAE} & \multirow{2}{*}{Abs. Rel.} & \multirow{2}{*}{Sq. Rel.} & \multirow{2}{*}{RMSE} & \multirow{2}{*}{RMSE (Log)} & Inlier Ratio & Inlier Ratio & Inlier Ratio \\
& & & & & & ($\lambda=1.25$) & ($\lambda=1.25^2$)& ($\lambda=1.25^3$)\\
\midrule
No Adaptation & 0.4339 & 0.1934 & 0.1418 & 0.6019 & 0.0953 & 0.7367 & 0.9618 & 0.9861 \\
Schneider et al.~\cite{batchnorm_update} & 0.5302 & 0.2057 & 0.2127 & 0.815 & 0.1221 & 0.6679 & 0.9089 & 0.9579 \\
Tent~\cite{tent} & 0.4278 & 0.1906 & 0.1388 & 0.5949 & 0.0943 & 0.7468 & 0.9624 & 0.9863 \\
Flip Consistency & 0.4203 & 0.1863 & 0.1341 & 0.5941 & 0.0917 & 0.7462 & 0.9619 & 0.9864 \\
Mask Consistency & 0.3976 & 0.1745 & 0.1232 & 0.5687 & 0.0883 & 0.7879 & 0.962 & 0.9866 \\
Photometric Consistency & 0.434 & 0.1958 & 0.1404 & 0.6027 & 0.0955 & 0.7235 & 0.9643 & 0.987 \\
Pseudo Labelling & 0.4087 & 0.1819 & 0.1281 & 0.5743 & 0.0909 & 0.7617 & 0.9637 & 0.9873 \\
Vanilla T\textsuperscript{2}Net~\cite{t2net} & 0.4182 & 0.1781 & 0.1334 & 0.6171 & 0.0921 & 0.7786 & 0.9547 & 0.9839 \\
CrDoCo~\cite{chen2019crdoco} & 0.4099 & 0.1797 & 0.126 & 0.5821 & 0.0907 & 0.7741 & 0.9603 & 0.9864 \\
Feature Consistency & 0.4152 & 0.1768 & 0.1306 & 0.6118 & 0.0915 & 0.7821 & 0.9551 & 0.984 \\
Ground-Truth Training & 0.3161 & 0.1411 & 0.0899 & 0.4893 & 0.0764 & 0.8621 & 0.9758 & 0.991 \\
Ours & 0.3245 & 0.1448 & 0.0928 & 0.4756 & 0.0779 & 0.8686 & 0.9714 & 0.989  \\
\bottomrule
\end{tabularx}
}
\caption{Offline adaptation using 5\% of the panorama images for training in the OmniScenes~\cite{piccolo} dataset.}
\end{table*}

    \smallskip

\begin{table*}[t]
\centering
\resizebox{0.9\linewidth}{!}{
\begin{tabularx}{2.5\columnwidth}{l|YYYYYYYY}
\toprule
\multirow{2}{*}{Method} & \multirow{2}{*}{MAE} & \multirow{2}{*}{Abs. Rel.} & \multirow{2}{*}{Sq. Rel.} & \multirow{2}{*}{RMSE} & \multirow{2}{*}{RMSE (Log)} & Inlier Ratio & Inlier Ratio & Inlier Ratio \\
& & & & & & ($\lambda=1.25$) & ($\lambda=1.25^2$)& ($\lambda=1.25^3$)\\
\midrule
No Adaptation & 0.4345 & 0.1951 & 0.1430 & 0.6029 & 0.0953 & 0.7335 & 0.9626 & 0.9866 \\
Schneider et al.~\cite{batchnorm_update} & 0.5317 & 0.2072 & 0.2144 & 0.8169 & 0.1220 & 0.6627 & 0.9087 & 0.9585 \\
Tent~\cite{tent} & 0.4280 & 0.192 & 0.1396 & 0.5957 & 0.0942 & 0.7455 & 0.9634 & 0.9868 \\
Flip Consistency & 0.4044 & 0.1808 & 0.1263 & 0.5743 & 0.0897 & 0.7631 & 0.9633 & 0.9872 \\
Mask Consistency & 0.4022 & 0.1775 & 0.1252 & 0.5732 & 0.0893 & 0.7834 & 0.9612 & 0.9867 \\
Photometric Consistency & 0.4253 & 0.1926 & 0.1367 & 0.5845 & 0.0933 & 0.7364 & 0.9659 & 0.9879 \\
Pseudo Labelling & 0.4167 & 0.1846 & 0.1311 & 0.5907 & 0.0916 & 0.7580 & 0.9630 & 0.9873 \\
Vanilla T\textsuperscript{2}Net~\cite{t2net} & 0.4210 & 0.1806 & 0.1344 & 0.6210 & 0.0927 & 0.7738 & 0.9536 & 0.9841 \\
CrDoCo~\cite{chen2019crdoco} & 0.4112 & 0.1814 & 0.1274 & 0.5850 & 0.0911 & 0.7719 & 0.9598 & 0.9865 \\
Feature Consistency & 0.4192 & 0.1775 & 0.1335 & 0.6233 & 0.0925 & 0.7794 & 0.9531 & 0.9836 \\
Ground-Truth Training & 0.2981 & 0.1363 & 0.0813 & 0.4543 & 0.0731 & 0.8754 & 0.9793 & 0.9923 \\
Ours & 0.3192 & 0.1434 & 0.0907 & 0.4674 & 0.0767 & 0.8732 & 0.9725 & 0.9896 \\ 
\bottomrule
\end{tabularx}
}
\caption{Offline adaptation using 10\% of the panorama images for training in the OmniScenes~\cite{piccolo} dataset.}
\end{table*}

    \smallskip

\begin{table*}[t]
\centering
\resizebox{0.9\linewidth}{!}{
\begin{tabularx}{2.5\columnwidth}{l|YYYYYYYY}
\toprule
\multirow{2}{*}{Method} & \multirow{2}{*}{MAE} & \multirow{2}{*}{Abs. Rel.} & \multirow{2}{*}{Sq. Rel.} & \multirow{2}{*}{RMSE} & \multirow{2}{*}{RMSE (Log)} & Inlier Ratio & Inlier Ratio & Inlier Ratio \\
& & & & & & ($\lambda=1.25$) & ($\lambda=1.25^2$)& ($\lambda=1.25^3$)\\
\midrule
No Adaptation & 0.4334 & 0.1946 & 0.1431 & 0.6030 & 0.0957 & 0.7362 & 0.9616 & 0.9863 \\
Schneider et al.~\cite{batchnorm_update} & 0.4053 & 0.1555 & 0.1368 & 0.7470 & 0.1028 & 0.8033 & 0.9487 & 0.9794 \\
Tent~\cite{tent} & 0.4198 & 0.1848 & 0.1355 & 0.6320 & 0.0955 & 0.7727 & 0.9608 & 0.9859 \\
Flip Consistency & 0.4700 & 0.1903 & 0.1628 & 0.8111 & 0.1059 & 0.7318 & 0.9372 & 0.9742 \\
Mask Consistency & 0.4898 & 0.2069 & 0.1705 & 0.8097 & 0.1095 & 0.6713 & 0.9324 & 0.9731 \\
Photometric Consistency & 0.4498 & 0.2083 & 0.1479 & 0.6656 & 0.1023 & 0.6615 & 0.9555 & 0.9862 \\
Pseudo Labelling & 0.4533 & 0.2043 & 0.1493 & 0.7110 & 0.1035 & 0.6910 & 0.9464 & 0.9801 \\
Vanilla T\textsuperscript{2}Net~\cite{t2net} & 0.4025 & 0.1767 & 0.1259 & 0.6345 & 0.0936 & 0.7909 & 0.9563 & 0.9831 \\
CrDoCo~\cite{chen2019crdoco} & 0.4989 & 0.2115 & 0.1779 & 0.8306 & 0.1117 & 0.6668 & 0.9311 & 0.9704 \\
Feature Consistency & 0.6594 & 0.2402 & 0.3025 & 1.1390 & 0.1546 & 0.5887 & 0.8267 & 0.9172 \\
Ground-Truth Training & 0.2243 & 0.0922 & 0.0622 & 0.4245 & 0.0619 & 0.9143 & 0.9801 & 0.9930 \\
Ours & 0.3382 & 0.1433 & 0.0989 & 0.5393 & 0.0816 & 0.8432 & 0.9667 & 0.9902
 \\
\bottomrule
\end{tabularx}
}
\caption{Online adaptation in dataset shift evaluated in the OmniScenes~\cite{piccolo} dataset.}
\end{table*}

    \smallskip

\begin{table*}[t]
\centering
\resizebox{0.9\linewidth}{!}{
\begin{tabularx}{2.5\columnwidth}{l|YYYYYYYY}
\toprule
\multirow{2}{*}{Method} & \multirow{2}{*}{MAE} & \multirow{2}{*}{Abs. Rel.} & \multirow{2}{*}{Sq. Rel.} & \multirow{2}{*}{RMSE} & \multirow{2}{*}{RMSE (Log)} & Inlier Ratio & Inlier Ratio & Inlier Ratio \\
& & & & & & ($\lambda=1.25$) & ($\lambda=1.25^2$)& ($\lambda=1.25^3$)\\
\midrule
No Adaptation & 0.3766 & 0.2117 & 0.1378 & 0.4868 & 0.0966 & 0.7060 & 0.9715 & 0.9893 \\
Schneider et al.~\cite{batchnorm_update} & 0.3611 & 0.1944 & 0.1115 & 0.4837 & 0.0894 & 0.7520 & 0.9797 & 0.9930 \\
Tent~\cite{tent} & 0.3495 & 0.1977 & 0.1215 & 0.4616 & 0.0938 & 0.7643 & 0.9740 & 0.9901 \\
Flip Consistency & 0.2823 & 0.1727 & 0.0833 & 0.3662 & 0.0850 & 0.8193 & 0.9782 & 0.9925 \\
Mask Consistency & 0.3134 & 0.1999 & 0.0948 & 0.3870 & 0.0940 & 0.7231 & 0.9710 & 0.9918 \\
Photometric Consistency & 0.3486 & 0.2066 & 0.1201 & 0.4373 & 0.0971 & 0.7083 & 0.9714 & 0.9895 \\
Pseudo Labelling & 0.3498 & 0.2166 & 0.1127 & 0.4254 & 0.0983 & 0.6855 & 0.9692 & 0.9910 \\
Vanilla T\textsuperscript{2}Net~\cite{t2net} & 0.3286 & 0.2126 & 0.1058 & 0.3930 & 0.0975 & 0.7163 & 0.9690 & 0.9911 \\
CrDoCo~\cite{chen2019crdoco} & 0.3268 & 0.2063 & 0.0998 & 0.4068 & 0.0964 & 0.7131 & 0.9682 & 0.9916 \\
Feature Consistency & 0.4863 & 0.2433 & 0.2117 & 0.7122 & 0.1478 & 0.5800 & 0.8350 & 0.9256 \\
Ground-Truth Training & 0.1409 & 0.0835 & 0.0355 & 0.2284 & 0.0548 & 0.9411 & 0.9863 & 0.9948 \\
Ours & 0.1971 & 0.1099 & 0.0498 & 0.3042 & 0.0650 & 0.9132 & 0.9848 & 0.9942 \\
\bottomrule
\end{tabularx}
}
\caption{Online adaptation in low lighting evaluated in the OmniScenes~\cite{piccolo} dataset..}
\end{table*}

\begin{table*}[t]
\centering
\resizebox{0.9\linewidth}{!}{
\begin{tabularx}{2.5\columnwidth}{l|YYYYYYYY}
\toprule
\multirow{2}{*}{Method} & \multirow{2}{*}{MAE} & \multirow{2}{*}{Abs. Rel.} & \multirow{2}{*}{Sq. Rel.} & \multirow{2}{*}{RMSE} & \multirow{2}{*}{RMSE (Log)} & Inlier Ratio & Inlier Ratio & Inlier Ratio \\
& & & & & & ($\lambda=1.25$) & ($\lambda=1.25^2$)& ($\lambda=1.25^3$)\\
\midrule
No Adaptation & 0.3929 & 0.2215 & 0.1412 & 0.4980 & 0.1000 & 0.6707 & 0.9686 & 0.9882 \\
Schneider et al.~\cite{batchnorm_update} & 0.3638 & 0.1952 & 0.1113 & 0.4854 & 0.0895 & 0.7459 & 0.9805 & 0.9934 \\
Tent~\cite{tent} & 0.3656 & 0.2072 & 0.1250 & 0.4733 & 0.0974 & 0.7315 & 0.9711 & 0.9891 \\
Flip Consistency & 0.2879 & 0.1727 & 0.0790 & 0.3757 & 0.0858 & 0.8123 & 0.9768 & 0.9919 \\
Mask Consistency & 0.3261 & 0.2037 & 0.0976 & 0.4063 & 0.0958 & 0.7104 & 0.9696 & 0.9913 \\
Photometric Consistency & 0.3948 & 0.2368 & 0.1348 & 0.4736 & 0.1054 & 0.5850 & 0.9678 & 0.9895 \\
Pseudo Labelling & 0.3400 & 0.2120 & 0.1041 & 0.4097 & 0.0973 & 0.7001 & 0.9695 & 0.9911 \\
Vanilla T\textsuperscript{2}Net~\cite{t2net} & 0.3381 & 0.2128 & 0.1056 & 0.4033 & 0.0968 & 0.7219 & 0.9720 & 0.9915 \\
CrDoCo~\cite{chen2019crdoco} & 0.3301 & 0.2085 & 0.0999 & 0.4066 & 0.0968 & 0.7103 & 0.9690 & 0.9914 \\
Feature Consistency & 0.4502 & 0.2350 & 0.1839 & 0.6507 & 0.1348 & 0.6048 & 0.8644 & 0.9497 \\
Ground-Truth Training & 0.1445 & 0.0850 & 0.0355 & 0.2338 & 0.0560 & 0.9359 & 0.9855 & 0.9944 \\
Ours & 0.2107 & 0.1154 & 0.0519 & 0.3228 & 0.0679 & 0.9006 & 0.9833 & 0.9936
 \\
\bottomrule
\end{tabularx}
}
\caption{Online adaptation in white balance change evaluated in the OmniScenes~\cite{piccolo} dataset..}
\end{table*}

\begin{table*}[t]
\centering
\resizebox{0.9\linewidth}{!}{
\begin{tabularx}{2.5\columnwidth}{l|YYYYYYYY}
\toprule
\multirow{2}{*}{Method} & \multirow{2}{*}{MAE} & \multirow{2}{*}{Abs. Rel.} & \multirow{2}{*}{Sq. Rel.} & \multirow{2}{*}{RMSE} & \multirow{2}{*}{RMSE (Log)} & Inlier Ratio & Inlier Ratio & Inlier Ratio \\
& & & & & & ($\lambda=1.25$) & ($\lambda=1.25^2$)& ($\lambda=1.25^3$)\\
\midrule
No Adaptation & 0.3782 & 0.2116 & 0.1269 & 0.4778 & 0.0946 & 0.7262 & 0.9754 & 0.9910 \\
Schneider et al.~\cite{batchnorm_update} & 0.3615 & 0.1941 & 0.1104 & 0.4831 & 0.0891 & 0.7509 & 0.9810 & 0.9934 \\
Tent~\cite{tent} & 0.3474 & 0.1957 & 0.1108 & 0.4477 & 0.0911 & 0.7835 & 0.9776 & 0.9917 \\
Flip Consistency & 0.3026 & 0.1886 & 0.0861 & 0.3696 & 0.0883 & 0.7824 & 0.9791 & 0.9930 \\
Mask Consistency & 0.3281 & 0.2068 & 0.0958 & 0.3980 & 0.0952 & 0.6991 & 0.9736 & 0.9927 \\
Photometric Consistency & 0.3681 & 0.2283 & 0.1267 & 0.4361 & 0.1012 & 0.6431 & 0.9734 & 0.9911 \\
Pseudo Labelling & 0.3248 & 0.2018 & 0.0946 & 0.3890 & 0.0920 & 0.7500 & 0.9768 & 0.9928 \\
Vanilla T\textsuperscript{2}Net~\cite{t2net} & 0.3031 & 0.1921 & 0.0883 & 0.3667 & 0.0896 & 0.7788 & 0.9782 & 0.9926 \\
CrDoCo~\cite{chen2019crdoco} & 0.3105 & 0.1954 & 0.0886 & 0.3855 & 0.0915 & 0.7581 & 0.9751 & 0.9926 \\
Feature Consistency & 0.3747 & 0.1998 & 0.1324 & 0.5403 & 0.1115 & 0.6917 & 0.9159 & 0.9758 \\
Ground-Truth Training & 0.1354 & 0.0799 & 0.0325 & 0.2215 & 0.0531 & 0.9453 & 0.9875 & 0.9952 \\
Ours & 0.1990 & 0.1080 & 0.0474 & 0.3112 & 0.0648 & 0.9142 & 0.9851 & 0.9942
 \\
\bottomrule
\end{tabularx}
}
\caption{Online adaptation in image gamma change evaluated in the OmniScenes~\cite{piccolo} dataset.}
\end{table*}

\begin{table*}[t]
\centering
\resizebox{0.9\linewidth}{!}{
\begin{tabularx}{2.5\columnwidth}{l|YYYYYYYY}
\toprule
\multirow{2}{*}{Method} & \multirow{2}{*}{MAE} & \multirow{2}{*}{Abs. Rel.} & \multirow{2}{*}{Sq. Rel.} & \multirow{2}{*}{RMSE} & \multirow{2}{*}{RMSE (Log)} & Inlier Ratio & Inlier Ratio & Inlier Ratio \\
& & & & & & ($\lambda=1.25$) & ($\lambda=1.25^2$)& ($\lambda=1.25^3$)\\
\midrule
No Adaptation & 0.5290 & 0.1680 & 0.1696 & 0.8141 & 0.0975 & 0.7440 & 0.9399 & 0.9789 \\
Schneider et al.~\cite{batchnorm_update} & 0.7638 & 0.2101 & 0.3221 & 1.3617 & 0.1702 & 0.5857 & 0.8289 & 0.9272 \\
Tent~\cite{tent} & 0.5366 & 0.1678 & 0.1726 & 0.8776 & 0.1014 & 0.7461 & 0.9370 & 0.9780 \\
Flip Consistency & 0.6313 & 0.1721 & 0.2220 & 1.0901 & 0.1132 & 0.7247 & 0.9035 & 0.9601 \\
Mask Consistency & 0.6255 & 0.1745 & 0.2131 & 1.0730 & 0.1093 & 0.7273 & 0.9085 & 0.9662 \\
Photometric Consistency & 0.5512 & 0.1768 & 0.1750 & 0.8885 & 0.1013 & 0.6995 & 0.9405 & 0.9815 \\
Pseudo Labelling & 0.5747 & 0.1737 & 0.1857 & 0.9581 & 0.1025 & 0.7324 & 0.9261 & 0.9764 \\
Vanilla T\textsuperscript{2}Net~\cite{t2net} & 0.6003 & 0.1687 & 0.2001 & 1.0290 & 0.1061 & 0.7483 & 0.9162 & 0.9690 \\
CrDoCo~\cite{chen2019crdoco} & 0.6517 & 0.1825 & 0.2295 & 1.1306 & 0.1132 & 0.7116 & 0.9027 & 0.9617 \\
Feature Consistency & 0.8238 & 0.2163 & 0.3541 & 1.4397 & 0.1496 & 0.6082 & 0.8331 & 0.9258 \\
Ground-Truth Training & 0.3663 & 0.1147 & 0.1058 & 0.6516 & 0.0739 & 0.8773 & 0.9708 & 0.9898 \\
Ours & 0.4790 & 0.1494 & 0.1435 & 0.7819 & 0.0911 & 0.8029 & 0.9510 & 0.9855
 \\
\bottomrule
\end{tabularx}
}
\caption{Online adaptation in large scenes evaluated in the OmniScenes~\cite{piccolo} dataset.}
\end{table*}

\begin{table*}[t]
\centering
\resizebox{0.9\linewidth}{!}{
\begin{tabularx}{2.5\columnwidth}{l|YYYYYYYY}
\toprule
\multirow{2}{*}{Method} & \multirow{2}{*}{MAE} & \multirow{2}{*}{Abs. Rel.} & \multirow{2}{*}{Sq. Rel.} & \multirow{2}{*}{RMSE} & \multirow{2}{*}{RMSE (Log)} & Inlier Ratio & Inlier Ratio & Inlier Ratio \\
& & & & & & ($\lambda=1.25$) & ($\lambda=1.25^2$)& ($\lambda=1.25^3$)\\
\midrule
No Adaptation & 0.2921 & 0.1454 & 0.0738 & 0.4064 & 0.0750 & 0.8674 & 0.9787 & 0.9931 \\
Schneider et al.~\cite{batchnorm_update} & 0.2907 & 0.1388 & 0.0691 & 0.4183 & 0.0718 & 0.8625 & 0.9874 & 0.9954 \\
Tent~\cite{tent} & 0.2862 & 0.1424 & 0.0710 & 0.4029 & 0.0752 & 0.8730 & 0.9794 & 0.9934 \\
Flip Consistency & 0.2898 & 0.1499 & 0.0699 & 0.3888 & 0.0758 & 0.8549 & 0.9832 & 0.9946 \\
Mask Consistency & 0.2459 & 0.1317 & 0.0540 & 0.3321 & 0.0693 & 0.8851 & 0.9863 & 0.9954 \\
Photometric Consistency & 0.2560 & 0.1302 & 0.0587 & 0.3583 & 0.0702 & 0.8889 & 0.9831 & 0.9943 \\
Pseudo Labelling & 0.2732 & 0.1407 & 0.0624 & 0.3699 & 0.0716 & 0.8783 & 0.9857 & 0.9953 \\
Vanilla T\textsuperscript{2}Net~\cite{t2net} & 0.2453 & 0.1328 & 0.0542 & 0.3300 & 0.0698 & 0.8819 & 0.9860 & 0.9953 \\
CrDoCo~\cite{chen2019crdoco} & 0.2353 & 0.1269 & 0.0503 & 0.3216 & 0.0676 & 0.8905 & 0.9863 & 0.9953 \\
Feature Consistency & 0.2665 & 0.1283 & 0.0606 & 0.3835 & 0.0763 & 0.8547 & 0.9759 & 0.9904 \\
Ground-Truth Training & 0.1809 & 0.0930 & 0.0343 & 0.2679 & 0.0562 & 0.9325 & 0.9877 & 0.9954 \\
Ours & 0.2121 & 0.1058 & 0.0428 & 0.3119 & 0.0624 & 0.9139 & 0.9857 & 0.9946
 \\
\bottomrule
\end{tabularx}
}
\caption{Online adaptation in small scenes evaluated in the OmniScenes~\cite{piccolo} dataset.}
\end{table*}

\begin{table*}[t]
\centering
\resizebox{0.9\linewidth}{!}{
\begin{tabularx}{2.5\columnwidth}{l|YYYYYYYY}
\toprule
\multirow{2}{*}{Method} & \multirow{2}{*}{MAE} & \multirow{2}{*}{Abs. Rel.} & \multirow{2}{*}{Sq. Rel.} & \multirow{2}{*}{RMSE} & \multirow{2}{*}{RMSE (Log)} & Inlier Ratio & Inlier Ratio & Inlier Ratio \\
& & & & & & ($\lambda=1.25$) & ($\lambda=1.25^2$)& ($\lambda=1.25^3$)\\
\midrule
No Adaptation & 0.4585 & 0.2720 & 0.2294 & 0.6489 & 0.1443 & 0.5798 & 0.8498 & 0.9426 \\
Schneider et al.~\cite{batchnorm_update} & 0.4867 & 0.2878 & 0.2346 & 0.6636 & 0.1491 & 0.5088 & 0.8310 & 0.9432 \\
Tent~\cite{tent} & 0.4419 & 0.2570 & 0.2021 & 0.6299 & 0.1413 & 0.5924 & 0.8583 & 0.9469 \\
Flip Consistency & 0.4128 & 0.2389 & 0.1609 & 0.6048 & 0.1270 & 0.6184 & 0.8907 & 0.9652 \\
Mask Consistency & 0.4368 & 0.2358 & 0.1746 & 0.6737 & 0.1352 & 0.6165 & 0.8678 & 0.9526 \\
Photometric Consistency & 0.4316 & 0.2574 & 0.1929 & 0.6076 & 0.1338 & 0.5979 & 0.8788 & 0.9593 \\
Pseudo Labelling & 0.4421 & 0.2413 & 0.1786 & 0.6687 & 0.1364 & 0.6013 & 0.8667 & 0.9536 \\
Vanilla T\textsuperscript{2}Net~\cite{t2net} & 0.4044 & 0.2565 & 0.1891 & 0.5642 & 0.1298 & 0.6314 & 0.8880 & 0.9613 \\
CrDoCo~\cite{chen2019crdoco} & 0.4214 & 0.2265 & 0.1668 & 0.6600 & 0.1314 & 0.6457 & 0.8741 & 0.9555 \\
Feature Consistency & 0.6067 & 0.2913 & 0.2990 & 0.9284 & 0.2001 & 0.4699 & 0.7231 & 0.8552 \\
Ground-Truth Training & 0.2604 & 0.1583 & 0.0864 & 0.3917 & 0.0916 & 0.7987 & 0.9488 & 0.9833 \\
Ours & 0.4089 & 0.2106 & 0.1486 & 0.6182 & 0.1324 & 0.6070 & 0.8686 & 0.9593
 \\
\bottomrule
\end{tabularx}
}
\caption{Online adaptation in camera rotations evaluated in the OmniScenes~\cite{piccolo} dataset.}
\end{table*}

\begin{table*}[t]
\centering
\resizebox{0.9\linewidth}{!}{
\begin{tabularx}{2.5\columnwidth}{l|YYYYYYYY}
\toprule
\multirow{2}{*}{Method} & \multirow{2}{*}{MAE} & \multirow{2}{*}{Abs. Rel.} & \multirow{2}{*}{Sq. Rel.} & \multirow{2}{*}{RMSE} & \multirow{2}{*}{RMSE (Log)} & Inlier Ratio & Inlier Ratio & Inlier Ratio \\
& & & & & & ($\lambda=1.25$) & ($\lambda=1.25^2$)& ($\lambda=1.25^3$)\\
\midrule
No Adaptation & 0.5029 & 0.2770 & 0.3114 & 0.7194 & 0.1768 & 0.5950 & 0.8021 & 0.8799 \\
Schneider et al.~\cite{batchnorm_update} & 0.3800 & 0.2071 & 0.1240 & 0.5075 & 0.0953 & 0.7070 & 0.9723 & 0.9914 \\
Tent~\cite{tent} & 0.4718 & 0.2585 & 0.2693 & 0.7245 & 0.1812 & 0.6205 & 0.8183 & 0.8916 \\
Flip Consistency & 0.3416 & 0.2064 & 0.1161 & 0.4584 & 0.1090 & 0.7121 & 0.9401 & 0.9753 \\
Mask Consistency & 0.3818 & 0.2004 & 0.1404 & 0.5899 & 0.1245 & 0.7092 & 0.9015 & 0.9578 \\
Photometric Consistency & 0.4544 & 0.2597 & 0.2660 & 0.6843 & 0.1672 & 0.6366 & 0.8445 & 0.9097 \\
Pseudo Labelling & 0.3274 & 0.1854 & 0.1078 & 0.4754 & 0.1070 & 0.7623 & 0.9339 & 0.9721 \\
Vanilla T\textsuperscript{2}Net~\cite{t2net} & 0.3324 & 0.2043 & 0.1369 & 0.4648 & 0.1126 & 0.7495 & 0.9298 & 0.9681 \\
CrDoCo~\cite{chen2019crdoco} & 0.3383 & 0.1929 & 0.1102 & 0.4906 & 0.1051 & 0.7404 & 0.9408 & 0.9781 \\
Feature Consistency & 0.4046 & 0.2115 & 0.1539 & 0.6142 & 0.1302 & 0.6660 & 0.8876 & 0.9531 \\
Ground-Truth Training & 0.1868 & 0.1096 & 0.0550 & 0.2947 & 0.0720 & 0.8907 & 0.9674 & 0.9860 \\
Ours & 0.2557 & 0.1349 & 0.0717 & 0.4037 & 0.0851 & 0.8445 & 0.9597 & 0.9837
 \\
\bottomrule
\end{tabularx}
}
\caption{Online adaptation in gaussian noise evaluated in the OmniScenes~\cite{piccolo} dataset.}
\end{table*}

\begin{table*}[t]
\centering
\resizebox{0.9\linewidth}{!}{
\begin{tabularx}{2.5\columnwidth}{l|YYYYYYYY}
\toprule
\multirow{2}{*}{Method} & \multirow{2}{*}{MAE} & \multirow{2}{*}{Abs. Rel.} & \multirow{2}{*}{Sq. Rel.} & \multirow{2}{*}{RMSE} & \multirow{2}{*}{RMSE (Log)} & Inlier Ratio & Inlier Ratio & Inlier Ratio \\
& & & & & & ($\lambda=1.25$) & ($\lambda=1.25^2$)& ($\lambda=1.25^3$)\\
\midrule
No Adaptation & 0.7473 & 0.4189 & 0.4784 & 0.9412 & 0.1649 & 0.3244 & 0.7849 & 0.9368 \\
Schneider et al.~\cite{batchnorm_update} & 0.3805 & 0.2064 & 0.1217 & 0.5048 & 0.0948 & 0.7144 & 0.9723 & 0.9923 \\
Tent~\cite{tent} & 0.6900 & 0.3872 & 0.4067 & 0.8798 & 0.1576 & 0.3752 & 0.8195 & 0.9481 \\
Flip Consistency & 0.4892 & 0.3025 & 0.2027 & 0.5750 & 0.1281 & 0.4454 & 0.9114 & 0.9793 \\
Mask Consistency & 0.4715 & 0.2995 & 0.1914 & 0.5531 & 0.1281 & 0.4464 & 0.9129 & 0.9799 \\
Photometric Consistency & 0.7913 & 0.4655 & 0.4944 & 0.9309 & 0.1776 & 0.1959 & 0.7345 & 0.9340 \\
Pseudo Labelling & 0.4980 & 0.3064 & 0.2038 & 0.5793 & 0.1286 & 0.4273 & 0.9164 & 0.9803 \\
Vanilla T\textsuperscript{2}Net~\cite{t2net} & 0.5771 & 0.3668 & 0.3141 & 0.6923 & 0.1511 & 0.4214 & 0.8409 & 0.9531 \\
CrDoCo~\cite{chen2019crdoco} & 0.4024 & 0.2534 & 0.1463 & 0.4898 & 0.1130 & 0.5797 & 0.9392 & 0.9852 \\
Feature Consistency & 0.4755 & 0.2377 & 0.1979 & 0.7094 & 0.1417 & 0.5922 & 0.8486 & 0.9376 \\
Ground-Truth Training & 0.2030 & 0.1171 & 0.0575 & 0.3034 & 0.0677 & 0.8789 & 0.9764 & 0.9925 \\
Ours & 0.3311 & 0.1876 & 0.1080 & 0.4455 & 0.0930 & 0.7160 & 0.9620 & 0.9905
 \\
\bottomrule
\end{tabularx}
}
\caption{Online adaptation in salt and pepper noise evaluated in the OmniScenes~\cite{piccolo} dataset.}
\end{table*}

\begin{table*}[t]
\centering
\resizebox{0.9\linewidth}{!}{
\begin{tabularx}{2.5\columnwidth}{l|YYYYYYYY}
\toprule
\multirow{2}{*}{Method} & \multirow{2}{*}{MAE} & \multirow{2}{*}{Abs. Rel.} & \multirow{2}{*}{Sq. Rel.} & \multirow{2}{*}{RMSE} & \multirow{2}{*}{RMSE (Log)} & Inlier Ratio & Inlier Ratio & Inlier Ratio \\
& & & & & & ($\lambda=1.25$) & ($\lambda=1.25^2$)& ($\lambda=1.25^3$)\\
\midrule
No Adaptation & 0.5285 & 0.2970 & 0.3467 & 0.7498 & 0.1787 & 0.5729 & 0.8000 & 0.8826 \\
Schneider et al.~\cite{batchnorm_update} & 0.3918 & 0.2119 & 0.1344 & 0.5313 & 0.0981 & 0.7048 & 0.9646 & 0.9890 \\
Tent~\cite{tent} & 0.4945 & 0.2753 & 0.2902 & 0.7334 & 0.1783 & 0.5988 & 0.8170 & 0.8958 \\
Flip Consistency & 0.3779 & 0.2323 & 0.1408 & 0.4878 & 0.1154 & 0.6493 & 0.9347 & 0.9751 \\
Mask Consistency & 0.3641 & 0.2137 & 0.1273 & 0.5021 & 0.1117 & 0.6906 & 0.9327 & 0.9764 \\
Photometric Consistency & 0.5642 & 0.3368 & 0.4919 & 0.8553 & 0.2010 & 0.5685 & 0.7775 & 0.8630 \\
Pseudo Labelling & 0.3761 & 0.2233 & 0.1510 & 0.5260 & 0.1182 & 0.6849 & 0.9232 & 0.9695 \\
Vanilla T\textsuperscript{2}Net~\cite{t2net} & 0.3691 & 0.2299 & 0.1603 & 0.4953 & 0.1169 & 0.6954 & 0.9246 & 0.9698 \\
CrDoCo~\cite{chen2019crdoco} & 0.3581 & 0.2093 & 0.1233 & 0.5006 & 0.1096 & 0.7097 & 0.9355 & 0.9771 \\
Feature Consistency & 0.4086 & 0.2218 & 0.1542 & 0.5971 & 0.1280 & 0.6413 & 0.8958 & 0.9611 \\
Ground-Truth Training & 0.2036 & 0.1194 & 0.0602 & 0.3150 & 0.0744 & 0.8745 & 0.9683 & 0.9878 \\
Ours & 0.2753 & 0.1509 & 0.0830 & 0.4160 & 0.0881 & 0.8233 & 0.9603 & 0.9850
 \\
\bottomrule
\end{tabularx}
}
\caption{Online adaptation in speckle noise evaluated in the OmniScenes~\cite{piccolo} dataset.}
\end{table*}
