# Supplementary material for: Calibrating Panoramic Depth Estimation for Practical Localization and Mapping
Source: arXiv:2308.14005 source file (2024-02-02)
Supplement: Supplementary file 3 [file supp_full_stanford.tex]

\begin{table*}[t]
\centering
\resizebox{0.9\linewidth}{!}{
\begin{tabularx}{2.5\columnwidth}{l|YYYYYYYY}
\toprule
\multirow{2}{*}{Method} & \multirow{2}{*}{MAE} & \multirow{2}{*}{Abs. Rel.} & \multirow{2}{*}{Sq. Rel.} & \multirow{2}{*}{RMSE} & \multirow{2}{*}{RMSE (Log)} & Inlier Ratio & Inlier Ratio & Inlier Ratio \\
& & & & & & ($\lambda=1.25$) & ($\lambda=1.25^2$)& ($\lambda=1.25^3$)\\
\midrule
No Adaptation & 0.4656 & 0.2533 & 0.2171 & 0.6551 & 0.1215 & 0.63 & 0.9077 & 0.9704 \\
Schneider et al.~\cite{batchnorm_update} & 0.5102 & 0.2684 & 0.2686 & 0.7714 & 0.1308 & 0.5776 & 0.8871 & 0.9632 \\
Tent~\cite{tent} & 0.4645 & 0.2527 & 0.2163 & 0.6537 & 0.1213 & 0.6314 & 0.908 & 0.9705 \\
Flip Consistency & 0.4586 & 0.2494 & 0.2085 & 0.6441 & 0.1207 & 0.6344 & 0.9091 & 0.9706 \\
Mask Consistency & 0.444 & 0.2426 & 0.1967 & 0.6271 & 0.118 & 0.6522 & 0.914 & 0.9722 \\
Photometric Consistency & 0.4674 & 0.2559 & 0.2188 & 0.6538 & 0.1218 & 0.6254 & 0.9071 & 0.9706 \\
Pseudo Labelling & 0.4476 & 0.2471 & 0.2006 & 0.6214 & 0.1179 & 0.6411 & 0.9133 & 0.9732 \\
Vanilla T\textsuperscript{2}Net~\cite{t2net} & 0.4404 & 0.2402 & 0.1944 & 0.6268 & 0.1183 & 0.6565 & 0.9136 & 0.9716 \\
CrDoCo~\cite{chen2019crdoco} & 0.444 & 0.2437 & 0.1971 & 0.6257 & 0.1181 & 0.6497 & 0.9134 & 0.9722 \\
Feature Consistency & 0.4374 & 0.2365 & 0.19 & 0.6223 & 0.1172 & 0.6611 & 0.9155 & 0.9722 \\
Ground-Truth Training & 0.4023 & 0.2234 & 0.1678 & 0.5646 & 0.1108 & 0.6903 & 0.9252 & 0.9762 \\
Ours & 0.4313 & 0.2365 & 0.1896 & 0.6057 & 0.1152 & 0.6652 & 0.9185 & 0.9744 \\
\bottomrule
\end{tabularx}
}
\caption{Offline adaptation using 5\% of the panorama images for training in the Stanford 2D-3D-S~\cite{stanford2d3d} dataset.}
\end{table*}

    \smallskip

\begin{table*}[t]
\centering
\resizebox{0.9\linewidth}{!}{
\begin{tabularx}{2.5\columnwidth}{l|YYYYYYYY}
\toprule
\multirow{2}{*}{Method} & \multirow{2}{*}{MAE} & \multirow{2}{*}{Abs. Rel.} & \multirow{2}{*}{Sq. Rel.} & \multirow{2}{*}{RMSE} & \multirow{2}{*}{RMSE (Log)} & Inlier Ratio & Inlier Ratio & Inlier Ratio \\
& & & & & & ($\lambda=1.25$) & ($\lambda=1.25^2$)& ($\lambda=1.25^3$)\\
\midrule
No Adaptation & 0.4601 & 0.2491 & 0.2136 & 0.6560 & 0.1217 & 0.6387 & 0.9091 & 0.9698 \\
Schneider et al.~\cite{batchnorm_update} & 0.4973 & 0.2618 & 0.2557 & 0.7548 & 0.1276 & 0.5865 & 0.8957 & 0.9662 \\
Tent~\cite{tent} & 0.4592 & 0.2486 & 0.2129 & 0.6549 & 0.1215 & 0.6398 & 0.9094 & 0.9699 \\
Flip Consistency & 0.4513 & 0.2461 & 0.2051 & 0.6383 & 0.1202 & 0.6435 & 0.9115 & 0.9706 \\
Mask Consistency & 0.4461 & 0.2411 & 0.2004 & 0.6419 & 0.1197 & 0.6554 & 0.9124 & 0.9702 \\
Photometric Consistency & 0.4623 & 0.2510 & 0.2152 & 0.6573 & 0.1220 & 0.6352 & 0.9085 & 0.9698 \\
Pseudo Labelling & 0.4505 & 0.2448 & 0.2038 & 0.6431 & 0.1206 & 0.6452 & 0.9108 & 0.9701 \\
Vanilla T\textsuperscript{2}Net~\cite{t2net} & 0.4430 & 0.2385 & 0.1983 & 0.6419 & 0.1198 & 0.6610 & 0.9120 & 0.9694 \\
CrDoCo~\cite{chen2019crdoco} & 0.4444 & 0.2419 & 0.1991 & 0.6362 & 0.1191 & 0.6537 & 0.9131 & 0.9711 \\
Feature Consistency & 0.4415 & 0.2378 & 0.1971 & 0.6385 & 0.1196 & 0.6618 & 0.9116 & 0.9693 \\
Ground-Truth Training & 0.4073 & 0.2255 & 0.1741 & 0.5789 & 0.1126 & 0.6881 & 0.9236 & 0.9749 \\
Ours & 0.4313 & 0.2350 & 0.1914 & 0.6134 & 0.1168 & 0.6686 & 0.9164 & 0.9722 \\
\bottomrule
\end{tabularx}
}
\caption{Offline adaptation using 10\% of the panorama images for training in the Stanford 2D-3D-S~\cite{stanford2d3d} dataset.}
\end{table*}

    \smallskip

\begin{table*}[t]
\centering
\resizebox{0.9\linewidth}{!}{
\begin{tabularx}{2.5\columnwidth}{l|YYYYYYYY}
\toprule
\multirow{2}{*}{Method} & \multirow{2}{*}{MAE} & \multirow{2}{*}{Abs. Rel.} & \multirow{2}{*}{Sq. Rel.} & \multirow{2}{*}{RMSE} & \multirow{2}{*}{RMSE (Log)} & Inlier Ratio & Inlier Ratio & Inlier Ratio \\
& & & & & & ($\lambda=1.25$) & ($\lambda=1.25^2$)& ($\lambda=1.25^3$)\\
\midrule
No Adaptation & 0.4538 & 0.2461 & 0.2069 & 0.6504 & 0.1208 & 0.6444 & 0.9113 & 0.9708 \\
Schneider et al.~\cite{batchnorm_update} & 0.4381 & 0.2351 & 0.1957 & 0.6793 & 0.1156 & 0.6446 & 0.9266 & 0.9780 \\
Tent~\cite{tent} & 0.4397 & 0.2361 & 0.1949 & 0.6680 & 0.1209 & 0.6683 & 0.9159 & 0.9718 \\
Flip Consistency & 0.3951 & 0.2253 & 0.1538 & 0.6183 & 0.1145 & 0.6785 & 0.9221 & 0.9750 \\
Mask Consistency & 0.4120 & 0.2333 & 0.1638 & 0.6594 & 0.1186 & 0.6552 & 0.9152 & 0.9709 \\
Photometric Consistency & 0.4752 & 0.2792 & 0.2150 & 0.6596 & 0.1277 & 0.5670 & 0.9030 & 0.9718 \\
Pseudo Labelling & 0.4038 & 0.2304 & 0.1608 & 0.6329 & 0.1165 & 0.6684 & 0.9186 & 0.9729 \\
Vanilla T\textsuperscript{2}Net~\cite{t2net} & 0.4017 & 0.2336 & 0.1683 & 0.6236 & 0.1166 & 0.6762 & 0.9156 & 0.9726 \\
CrDoCo~\cite{chen2019crdoco} & 0.4091 & 0.2313 & 0.1644 & 0.6626 & 0.1175 & 0.6654 & 0.9137 & 0.9714 \\
Feature Consistency & 0.6116 & 0.2687 & 0.3168 & 1.0522 & 0.1906 & 0.5360 & 0.7803 & 0.8794 \\
Ground-Truth Training & 0.2624 & 0.1415 & 0.0921 & 0.4524 & 0.0866 & 0.8366 & 0.9585 & 0.9860 \\
Ours & 0.2994 & 0.1594 & 0.1136 & 0.5008 & 0.0944 & 0.8086 & 0.9511 & 0.9824
 \\
\bottomrule
\end{tabularx}
}
\caption{Online adaptation in dataset shift evaluated in the Stanford 2D-3D-S~\cite{stanford2d3d} dataset.}
\end{table*}

    \smallskip

\begin{table*}[t]
\centering
\resizebox{0.9\linewidth}{!}{
\begin{tabularx}{2.5\columnwidth}{l|YYYYYYYY}
\toprule
\multirow{2}{*}{Method} & \multirow{2}{*}{MAE} & \multirow{2}{*}{Abs. Rel.} & \multirow{2}{*}{Sq. Rel.} & \multirow{2}{*}{RMSE} & \multirow{2}{*}{RMSE (Log)} & Inlier Ratio & Inlier Ratio & Inlier Ratio \\
& & & & & & ($\lambda=1.25$) & ($\lambda=1.25^2$)& ($\lambda=1.25^3$)\\
\midrule
No Adaptation & 0.4018 & 0.2295 & 0.1645 & 0.5567 & 0.1157 & 0.6505 & 0.9194 & 0.9743 \\
Schneider et al.~\cite{batchnorm_update} & 0.4826 & 0.2759 & 0.2379 & 0.6949 & 0.1263 & 0.5577 & 0.9031 & 0.9725 \\
Tent~\cite{tent} & 0.3910 & 0.2225 & 0.1565 & 0.5652 & 0.1157 & 0.6682 & 0.9220 & 0.9749 \\
Flip Consistency & 0.3391 & 0.2086 & 0.1213 & 0.4775 & 0.1091 & 0.7039 & 0.9281 & 0.9774 \\
Mask Consistency & 0.3427 & 0.2140 & 0.1234 & 0.4817 & 0.1100 & 0.6942 & 0.9258 & 0.9769 \\
Photometric Consistency & 0.3874 & 0.2238 & 0.1527 & 0.5597 & 0.1188 & 0.6626 & 0.9179 & 0.9720 \\
Pseudo Labelling & 0.3671 & 0.2306 & 0.1411 & 0.5012 & 0.1136 & 0.6662 & 0.9213 & 0.9765 \\
Vanilla T\textsuperscript{2}Net~\cite{t2net} & 0.3670 & 0.2360 & 0.1464 & 0.4988 & 0.1158 & 0.6636 & 0.9150 & 0.9735 \\
CrDoCo~\cite{chen2019crdoco} & 0.3475 & 0.2109 & 0.1240 & 0.5055 & 0.1116 & 0.6933 & 0.9216 & 0.9751 \\
Feature Consistency & 0.4633 & 0.2501 & 0.2024 & 0.7093 & 0.1484 & 0.5870 & 0.8515 & 0.9350 \\
Ground-Truth Training & 0.2728 & 0.1594 & 0.0853 & 0.4119 & 0.0932 & 0.7954 & 0.9498 & 0.9851 \\
Ours & 0.2995 & 0.1712 & 0.1001 & 0.4517 & 0.0987 & 0.7696 & 0.9440 & 0.9815 \\
\bottomrule
\end{tabularx}
}
\caption{Online adaptation in low lighting evaluated in the Stanford 2D-3D-S~\cite{stanford2d3d} dataset..}
\end{table*}

\begin{table*}[t]
\centering
\resizebox{0.9\linewidth}{!}{
\begin{tabularx}{2.5\columnwidth}{l|YYYYYYYY}
\toprule
\multirow{2}{*}{Method} & \multirow{2}{*}{MAE} & \multirow{2}{*}{Abs. Rel.} & \multirow{2}{*}{Sq. Rel.} & \multirow{2}{*}{RMSE} & \multirow{2}{*}{RMSE (Log)} & Inlier Ratio & Inlier Ratio & Inlier Ratio \\
& & & & & & ($\lambda=1.25$) & ($\lambda=1.25^2$)& ($\lambda=1.25^3$)\\
\midrule
No Adaptation & 0.4484 & 0.2503 & 0.1943 & 0.6187 & 0.1289 & 0.6043 & 0.8947 & 0.9617 \\
Schneider et al.~\cite{batchnorm_update} & 0.4819 & 0.2749 & 0.2358 & 0.6904 & 0.1259 & 0.5581 & 0.9036 & 0.9731 \\
Tent~\cite{tent} & 0.4364 & 0.2426 & 0.1856 & 0.6328 & 0.1305 & 0.6231 & 0.8982 & 0.9622 \\
Flip Consistency & 0.3763 & 0.2190 & 0.1448 & 0.5630 & 0.1237 & 0.6775 & 0.9015 & 0.9626 \\
Mask Consistency & 0.3567 & 0.2250 & 0.1324 & 0.4933 & 0.1130 & 0.6819 & 0.9193 & 0.9755 \\
Photometric Consistency & 0.4583 & 0.2692 & 0.2000 & 0.6268 & 0.1314 & 0.5745 & 0.8938 & 0.9657 \\
Pseudo Labelling & 0.4116 & 0.2579 & 0.1670 & 0.5454 & 0.1225 & 0.6046 & 0.9069 & 0.9725 \\
Vanilla T\textsuperscript{2}Net~\cite{t2net} & 0.3934 & 0.2481 & 0.1597 & 0.5294 & 0.1200 & 0.6352 & 0.9087 & 0.9729 \\
CrDoCo~\cite{chen2019crdoco} & 0.3506 & 0.2190 & 0.1276 & 0.4926 & 0.1119 & 0.6902 & 0.9202 & 0.9761 \\
Feature Consistency & 0.5548 & 0.2730 & 0.2651 & 0.8570 & 0.1847 & 0.5144 & 0.7729 & 0.8830 \\
Ground-Truth Training & 0.2680 & 0.1574 & 0.0842 & 0.4079 & 0.0921 & 0.8039 & 0.9501 & 0.9849 \\
Ours & 0.3208 & 0.1779 & 0.1121 & 0.4968 & 0.1084 & 0.7516 & 0.9292 & 0.9736
 \\
\bottomrule
\end{tabularx}
}
\caption{Online adaptation in white balance change evaluated in the Stanford 2D-3D-S~\cite{stanford2d3d} dataset.}
\end{table*}

\begin{table*}[t]
\centering
\resizebox{0.9\linewidth}{!}{
\begin{tabularx}{2.5\columnwidth}{l|YYYYYYYY}
\toprule
\multirow{2}{*}{Method} & \multirow{2}{*}{MAE} & \multirow{2}{*}{Abs. Rel.} & \multirow{2}{*}{Sq. Rel.} & \multirow{2}{*}{RMSE} & \multirow{2}{*}{RMSE (Log)} & Inlier Ratio & Inlier Ratio & Inlier Ratio \\
& & & & & & ($\lambda=1.25$) & ($\lambda=1.25^2$)& ($\lambda=1.25^3$)\\
\midrule
No Adaptation & 0.4480 & 0.2630 & 0.2045 & 0.6001 & 0.1214 & 0.6096 & 0.9060 & 0.9729 \\
Schneider et al.~\cite{batchnorm_update} & 0.4787 & 0.2730 & 0.2278 & 0.6811 & 0.1247 & 0.5567 & 0.9056 & 0.9743 \\
Tent~\cite{tent} & 0.4306 & 0.2524 & 0.1906 & 0.5968 & 0.1201 & 0.6343 & 0.9117 & 0.9745 \\
Flip Consistency & 0.3722 & 0.2373 & 0.1459 & 0.4994 & 0.1144 & 0.6608 & 0.9186 & 0.9767 \\
Mask Consistency & 0.3439 & 0.2207 & 0.1275 & 0.4743 & 0.1098 & 0.6949 & 0.9245 & 0.9777 \\
Photometric Consistency & 0.5021 & 0.3105 & 0.2447 & 0.6446 & 0.1357 & 0.5093 & 0.8789 & 0.9662 \\
Pseudo Labelling & 0.3923 & 0.2499 & 0.1577 & 0.5182 & 0.1178 & 0.6302 & 0.9145 & 0.9757 \\
Vanilla T\textsuperscript{2}Net~\cite{t2net} & 0.3835 & 0.2490 & 0.1601 & 0.5140 & 0.1187 & 0.6445 & 0.9090 & 0.9732 \\
CrDoCo~\cite{chen2019crdoco} & 0.3575 & 0.2325 & 0.1391 & 0.4880 & 0.1137 & 0.6727 & 0.9164 & 0.9759 \\
Feature Consistency & 0.4370 & 0.2273 & 0.1832 & 0.6742 & 0.1415 & 0.6208 & 0.8598 & 0.9396 \\
Ground-Truth Training & 0.2600 & 0.1526 & 0.0836 & 0.4019 & 0.0900 & 0.8167 & 0.9527 & 0.9854 \\
Ours & 0.2887 & 0.1678 & 0.0993 & 0.4387 & 0.0956 & 0.7895 & 0.9468 & 0.9826
 \\
\bottomrule
\end{tabularx}
}
\caption{Online adaptation in image gamma change evaluated in the Stanford 2D-3D-S~\cite{stanford2d3d} dataset.}
\end{table*}

\begin{table*}[t]
\centering
\resizebox{0.9\linewidth}{!}{
\begin{tabularx}{2.5\columnwidth}{l|YYYYYYYY}
\toprule
\multirow{2}{*}{Method} & \multirow{2}{*}{MAE} & \multirow{2}{*}{Abs. Rel.} & \multirow{2}{*}{Sq. Rel.} & \multirow{2}{*}{RMSE} & \multirow{2}{*}{RMSE (Log)} & Inlier Ratio & Inlier Ratio & Inlier Ratio \\
& & & & & & ($\lambda=1.25$) & ($\lambda=1.25^2$)& ($\lambda=1.25^3$)\\
\midrule
No Adaptation & 0.4477 & 0.2187 & 0.2015 & 0.6987 & 0.1164 & 0.7078 & 0.9259 & 0.9698 \\
Schneider et al.~\cite{batchnorm_update} & 0.3996 & 0.1865 & 0.1607 & 0.6796 & 0.1048 & 0.7645 & 0.9473 & 0.9806 \\
Tent~\cite{tent} & 0.4541 & 0.2178 & 0.2011 & 0.7520 & 0.1204 & 0.7067 & 0.9253 & 0.9696 \\
Flip Consistency & 0.4345 & 0.2180 & 0.1738 & 0.7062 & 0.1110 & 0.7038 & 0.9382 & 0.9784 \\
Mask Consistency & 0.4330 & 0.2170 & 0.1749 & 0.7296 & 0.1110 & 0.7044 & 0.9361 & 0.9776 \\
Photometric Consistency & 0.4519 & 0.2170 & 0.1975 & 0.7504 & 0.1214 & 0.6990 & 0.9260 & 0.9686 \\
Pseudo Labelling & 0.4341 & 0.2070 & 0.1745 & 0.7638 & 0.1136 & 0.7193 & 0.9303 & 0.9734 \\
Vanilla T\textsuperscript{2}Net~\cite{t2net} & 0.4243 & 0.2060 & 0.1698 & 0.7484 & 0.1096 & 0.7282 & 0.9350 & 0.9763 \\
CrDoCo~\cite{chen2019crdoco} & 0.4212 & 0.2017 & 0.1665 & 0.7592 & 0.1082 & 0.7390 & 0.9356 & 0.9767 \\
Feature Consistency & 0.5788 & 0.2286 & 0.2871 & 1.1030 & 0.1693 & 0.6357 & 0.8420 & 0.9113 \\
Ground-Truth Training & 0.3121 & 0.1561 & 0.1243 & 0.5452 & 0.0894 & 0.8356 & 0.9605 & 0.9852 \\
Ours & 0.3471 & 0.1727 & 0.1423 & 0.5803 & 0.0960 & 0.8036 & 0.9546 & 0.9829
 \\
\bottomrule
\end{tabularx}
}
\caption{Online adaptation in large scenes evaluated in the Stanford 2D-3D-S~\cite{stanford2d3d} dataset.}
\end{table*}

\begin{table*}[t]
\centering
\resizebox{0.9\linewidth}{!}{
\begin{tabularx}{2.5\columnwidth}{l|YYYYYYYY}
\toprule
\multirow{2}{*}{Method} & \multirow{2}{*}{MAE} & \multirow{2}{*}{Abs. Rel.} & \multirow{2}{*}{Sq. Rel.} & \multirow{2}{*}{RMSE} & \multirow{2}{*}{RMSE (Log)} & Inlier Ratio & Inlier Ratio & Inlier Ratio \\
& & & & & & ($\lambda=1.25$) & ($\lambda=1.25^2$)& ($\lambda=1.25^3$)\\
\midrule
No Adaptation & 0.3692 & 0.2702 & 0.1673 & 0.4963 & 0.1289 & 0.5536 & 0.8942 & 0.9700 \\
Schneider et al.~\cite{batchnorm_update} & 0.7259 & 0.5169 & 0.5504 & 0.9410 & 0.1914 & 0.1590 & 0.6832 & 0.9222 \\
Tent~\cite{tent} & 0.3686 & 0.2684 & 0.1670 & 0.5025 & 0.1292 & 0.5605 & 0.8937 & 0.9693 \\
Flip Consistency & 0.3494 & 0.2575 & 0.1489 & 0.4742 & 0.1277 & 0.5780 & 0.8986 & 0.9681 \\
Mask Consistency & 0.3504 & 0.2614 & 0.1492 & 0.4681 & 0.1254 & 0.5726 & 0.9052 & 0.9717 \\
Photometric Consistency & 0.3900 & 0.2870 & 0.1836 & 0.5210 & 0.1318 & 0.5234 & 0.8856 & 0.9683 \\
Pseudo Labelling & 0.3788 & 0.2817 & 0.1737 & 0.5015 & 0.1298 & 0.5329 & 0.8933 & 0.9700 \\
Vanilla T\textsuperscript{2}Net~\cite{t2net} & 0.3598 & 0.2692 & 0.1584 & 0.4775 & 0.1271 & 0.5572 & 0.9006 & 0.9705 \\
CrDoCo~\cite{chen2019crdoco} & 0.3441 & 0.2565 & 0.1442 & 0.4637 & 0.1269 & 0.5813 & 0.8997 & 0.9684 \\
Feature Consistency & 0.3518 & 0.2558 & 0.1492 & 0.4838 & 0.1312 & 0.5715 & 0.8899 & 0.9635 \\
Ground-Truth Training & 0.3224 & 0.2387 & 0.1324 & 0.4428 & 0.1204 & 0.6365 & 0.9131 & 0.9731 \\
Ours & 0.3380 & 0.2485 & 0.1400 & 0.4612 & 0.1240 & 0.6030 & 0.9069 & 0.9717
 \\
\bottomrule
\end{tabularx}
}
\caption{Online adaptation in small scenes evaluated in the Stanford 2D-3D-S~\cite{stanford2d3d} dataset.}
\end{table*}

\begin{table*}[t]
\centering
\resizebox{0.9\linewidth}{!}{
\begin{tabularx}{2.5\columnwidth}{l|YYYYYYYY}
\toprule
\multirow{2}{*}{Method} & \multirow{2}{*}{MAE} & \multirow{2}{*}{Abs. Rel.} & \multirow{2}{*}{Sq. Rel.} & \multirow{2}{*}{RMSE} & \multirow{2}{*}{RMSE (Log)} & Inlier Ratio & Inlier Ratio & Inlier Ratio \\
& & & & & & ($\lambda=1.25$) & ($\lambda=1.25^2$)& ($\lambda=1.25^3$)\\
\midrule
No Adaptation & 0.6338 & 0.4173 & 0.5105 & 0.8961 & 0.1883 & 0.4565 & 0.7385 & 0.8736 \\
Schneider et al.~\cite{batchnorm_update} & 0.6689 & 0.4128 & 0.5905 & 1.0118 & 0.1957 & 0.4283 & 0.7307 & 0.8763 \\
Tent~\cite{tent} & 0.6140 & 0.4044 & 0.4817 & 0.8734 & 0.1863 & 0.4710 & 0.7482 & 0.8805 \\
Flip Consistency & 0.5165 & 0.3283 & 0.2912 & 0.7463 & 0.1654 & 0.5099 & 0.7931 & 0.9093 \\
Mask Consistency & 0.5241 & 0.3456 & 0.3090 & 0.7420 & 0.1666 & 0.5014 & 0.7883 & 0.9060 \\
Photometric Consistency & 0.7020 & 0.4857 & 0.6141 & 0.9436 & 0.2006 & 0.4037 & 0.6973 & 0.8547 \\
Pseudo Labelling & 0.5337 & 0.3482 & 0.3172 & 0.7543 & 0.1689 & 0.4933 & 0.7826 & 0.9045 \\
Vanilla T\textsuperscript{2}Net~\cite{t2net} & 0.5671 & 0.4031 & 0.4120 & 0.7711 & 0.1782 & 0.4838 & 0.7641 & 0.8876 \\
CrDoCo~\cite{chen2019crdoco} & 0.4875 & 0.3064 & 0.2586 & 0.7175 & 0.1576 & 0.5402 & 0.8119 & 0.9189 \\
Feature Consistency & 0.6049 & 0.3223 & 0.3282 & 0.9144 & 0.2048 & 0.4404 & 0.7076 & 0.8517 \\
Ground-Truth Training & 0.4140 & 0.2637 & 0.2149 & 0.6145 & 0.1382 & 0.6188 & 0.8560 & 0.9437 \\
Ours & 0.4910 & 0.2778 & 0.2513 & 0.7496 & 0.1659 & 0.5379 & 0.7986 & 0.9162
 \\
\bottomrule
\end{tabularx}
}
\caption{Online adaptation in camera rotations evaluated in the Stanford 2D-3D-S~\cite{stanford2d3d} dataset.}
\end{table*}

\begin{table*}[t]
\centering
\resizebox{0.9\linewidth}{!}{
\begin{tabularx}{2.5\columnwidth}{l|YYYYYYYY}
\toprule
\multirow{2}{*}{Method} & \multirow{2}{*}{MAE} & \multirow{2}{*}{Abs. Rel.} & \multirow{2}{*}{Sq. Rel.} & \multirow{2}{*}{RMSE} & \multirow{2}{*}{RMSE (Log)} & Inlier Ratio & Inlier Ratio & Inlier Ratio \\
& & & & & & ($\lambda=1.25$) & ($\lambda=1.25^2$)& ($\lambda=1.25^3$)\\
\midrule
No Adaptation & 0.5816 & 0.2848 & 0.3196 & 0.8809 & 0.2088 & 0.5158 & 0.7474 & 0.8531 \\
Schneider et al.~\cite{batchnorm_update} & 0.5049 & 0.2948 & 0.2788 & 0.7356 & 0.1354 & 0.5389 & 0.8807 & 0.9617 \\
Tent~\cite{tent} & 0.5788 & 0.2808 & 0.3131 & 0.9297 & 0.2143 & 0.5220 & 0.7478 & 0.8540 \\
Flip Consistency & 0.5882 & 0.2802 & 0.3002 & 0.9428 & 0.2032 & 0.5052 & 0.7474 & 0.8617 \\
Mask Consistency & 0.7381 & 0.3376 & 0.4076 & 1.1113 & 0.2568 & 0.3664 & 0.6149 & 0.7674 \\
Photometric Consistency & 0.4515 & 0.2441 & 0.2110 & 0.7100 & 0.1573 & 0.6191 & 0.8474 & 0.9269 \\
Pseudo Labelling & 0.5162 & 0.2587 & 0.2430 & 0.8323 & 0.1755 & 0.5605 & 0.8016 & 0.9005 \\
Vanilla T\textsuperscript{2}Net~\cite{t2net} & 0.4390 & 0.2497 & 0.2102 & 0.6776 & 0.1487 & 0.6234 & 0.8554 & 0.9349 \\
CrDoCo~\cite{chen2019crdoco} & 0.6525 & 0.3030 & 0.3396 & 1.0192 & 0.2214 & 0.4432 & 0.6924 & 0.8277 \\
Feature Consistency & 0.4787 & 0.2518 & 0.2171 & 0.7482 & 0.1605 & 0.5882 & 0.8276 & 0.9187 \\
Ground-Truth Training & 0.3183 & 0.1869 & 0.1206 & 0.4952 & 0.1109 & 0.7418 & 0.9176 & 0.9701 \\
Ours & 0.4091 & 0.2044 & 0.1651 & 0.6682 & 0.1417 & 0.6495 & 0.8719 & 0.9427
 \\
\bottomrule
\end{tabularx}
}
\caption{Online adaptation in gaussian noise evaluated in the Stanford 2D-3D-S~\cite{stanford2d3d} dataset.}
\end{table*}

\begin{table*}[t]
\centering
\resizebox{0.9\linewidth}{!}{
\begin{tabularx}{2.5\columnwidth}{l|YYYYYYYY}
\toprule
\multirow{2}{*}{Method} & \multirow{2}{*}{MAE} & \multirow{2}{*}{Abs. Rel.} & \multirow{2}{*}{Sq. Rel.} & \multirow{2}{*}{RMSE} & \multirow{2}{*}{RMSE (Log)} & Inlier Ratio & Inlier Ratio & Inlier Ratio \\
& & & & & & ($\lambda=1.25$) & ($\lambda=1.25^2$)& ($\lambda=1.25^3$)\\
\midrule
No Adaptation & 0.8215 & 0.4977 & 0.7425 & 1.1088 & 0.1973 & 0.3717 & 0.6989 & 0.8608 \\
Schneider et al.~\cite{batchnorm_update} & 0.5000 & 0.2864 & 0.2689 & 0.7428 & 0.1341 & 0.5560 & 0.8826 & 0.9641 \\
Tent~\cite{tent} & 0.7739 & 0.4674 & 0.6664 & 1.0653 & 0.1916 & 0.3970 & 0.7241 & 0.8759 \\
Flip Consistency & 0.4477 & 0.2872 & 0.2146 & 0.6100 & 0.1353 & 0.5787 & 0.8684 & 0.9546 \\
Mask Consistency & 0.4869 & 0.3141 & 0.2554 & 0.6591 & 0.1445 & 0.5340 & 0.8458 & 0.9437 \\
Photometric Consistency & 0.9862 & 0.6152 & 1.0352 & 1.2827 & 0.2288 & 0.2971 & 0.6131 & 0.7955 \\
Pseudo Labelling & 0.4995 & 0.3226 & 0.2622 & 0.6586 & 0.1451 & 0.5136 & 0.8429 & 0.9453 \\
Vanilla T\textsuperscript{2}Net~\cite{t2net} & 0.6522 & 0.4365 & 0.4794 & 0.8433 & 0.1797 & 0.4222 & 0.7406 & 0.8938 \\
CrDoCo~\cite{chen2019crdoco} & 0.4263 & 0.2697 & 0.1957 & 0.6018 & 0.1323 & 0.6111 & 0.8732 & 0.9557 \\
Feature Consistency & 0.5416 & 0.2721 & 0.2674 & 0.8473 & 0.1814 & 0.5372 & 0.7844 & 0.8905 \\
Ground-Truth Training & 0.3294 & 0.1957 & 0.1308 & 0.4940 & 0.1077 & 0.7434 & 0.9217 & 0.9741 \\
Ours & 0.3843 & 0.2290 & 0.1690 & 0.5610 & 0.1189 & 0.6806 & 0.9031 & 0.9670
 \\
\bottomrule
\end{tabularx}
}
\caption{Online adaptation in salt and pepper noise evaluated in the Stanford 2D-3D-S~\cite{stanford2d3d} dataset.}
\end{table*}

\begin{table*}[t]
\centering
\resizebox{0.9\linewidth}{!}{
\begin{tabularx}{2.5\columnwidth}{l|YYYYYYYY}
\toprule
\multirow{2}{*}{Method} & \multirow{2}{*}{MAE} & \multirow{2}{*}{Abs. Rel.} & \multirow{2}{*}{Sq. Rel.} & \multirow{2}{*}{RMSE} & \multirow{2}{*}{RMSE (Log)} & Inlier Ratio & Inlier Ratio & Inlier Ratio \\
& & & & & & ($\lambda=1.25$) & ($\lambda=1.25^2$)& ($\lambda=1.25^3$)\\
\midrule
No Adaptation & 0.5291 & 0.2777 & 0.2937 & 0.7796 & 0.1783 & 0.5324 & 0.7877 & 0.8992 \\
Schneider et al.~\cite{batchnorm_update} & 0.5032 & 0.2953 & 0.2651 & 0.7229 & 0.1342 & 0.5266 & 0.8850 & 0.9642 \\
Tent~\cite{tent} & 0.5250 & 0.2719 & 0.2807 & 0.8240 & 0.1824 & 0.5404 & 0.7918 & 0.9003 \\
Flip Consistency & 0.6716 & 0.3124 & 0.3487 & 1.0187 & 0.2264 & 0.3972 & 0.6693 & 0.8278 \\
Mask Consistency & 0.5444 & 0.2713 & 0.2576 & 0.8487 & 0.1760 & 0.5043 & 0.7904 & 0.9045 \\
Photometric Consistency & 0.4359 & 0.2632 & 0.2325 & 0.6427 & 0.1417 & 0.6097 & 0.8771 & 0.9494 \\
Pseudo Labelling & 0.4622 & 0.2503 & 0.2096 & 0.7200 & 0.1507 & 0.5853 & 0.8496 & 0.9368 \\
Vanilla T\textsuperscript{2}Net~\cite{t2net} & 0.4258 & 0.2532 & 0.2073 & 0.6372 & 0.1400 & 0.6183 & 0.8751 & 0.9496 \\
CrDoCo~\cite{chen2019crdoco} & 0.5459 & 0.2699 & 0.2550 & 0.8597 & 0.1752 & 0.5037 & 0.7910 & 0.9050 \\
Feature Consistency & 0.4766 & 0.2497 & 0.2181 & 0.7474 & 0.1582 & 0.5828 & 0.8321 & 0.9230 \\
Ground-Truth Training & 0.3062 & 0.1829 & 0.1178 & 0.4704 & 0.1052 & 0.7588 & 0.9307 & 0.9756 \\
Ours & 0.3375 & 0.1886 & 0.1266 & 0.5322 & 0.1125 & 0.7215 & 0.9218 & 0.9716
 \\
\bottomrule
\end{tabularx}
}
\caption{Online adaptation in speckle noise evaluated in the Stanford 2D-3D-S~\cite{stanford2d3d} dataset.}
\end{table*}
